# Supplementary material for: FoodPuzzle: Developing Large Language Model Agents as Flavor Scientists
Source: arXiv:2409.12832 source file (2024-10-07)
Supplement: Supplementary file 1 [file appendix.tex]

\section{Dataset Statistics}
\label{data_statistics}
Figure \ref{fig:molecule_nums_statistics} reveals that the majority of food entities are associated with a relatively small number of molecules, while a few entities have a significantly higher number of associated molecules. 
\begin{figure}[t]
    \centering
    \includegraphics[width=0.5\textwidth]{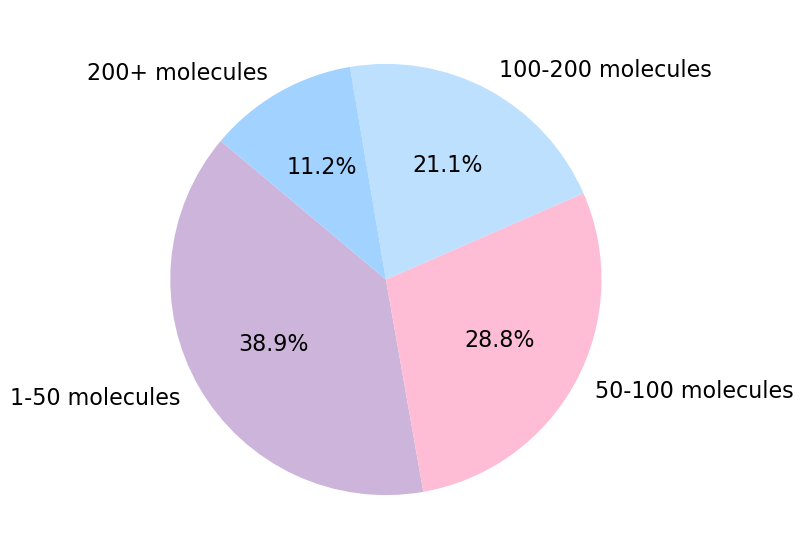}
    \caption{Distribution of the number of flavor molecules in the \datasetname dataset. The majority of foods (67.8\%) contain fewer than 100 flavor molecules. A smaller proportion of foods (32.2\%) contain more than 100 flavor molecules.}
    \label{fig:molecule_nums_statistics}
\end{figure}
% \begin{figure}[t]
%     \centering
%     \includegraphics[width=0.5\textwidth]{figs/association_rules_graph.png}
%     \caption{Graph-based visualization of association rules showing relationships between molecules. Circle size represents support values, color intensity indicates lift values, and arrows indicate the direction of the rules.}
%     \label{fig:association_rules}
% \end{figure}

\section{Prompt Details}
\label{apdx:prompt_details}

Figure \ref{fig:foundation_llms_prompts}, and Figure \ref{fig:icl_prompts} show the prompt details that we interact with the Foundation LLMs. Figure \ref{fig:MFP_auto_system_prompt}, Figure \ref{fig:MFP_auto_scientist_prompt}, Figure \ref{fig:MFP_auto_reviewer_prompt}, Figure \ref{fig:MPC_auto_system_prompt}, Figure \ref{fig:MPC_auto_scientist_prompt}, and Figure \ref{fig:MPC_auto_reviewer_prompt} show prompts used for Autonomous Scientific Agent.

\begin{figure}[htbp]
    \centering
    \begin{subfigure}[b]{0.5\textwidth}
        \includegraphics[width=\textwidth]{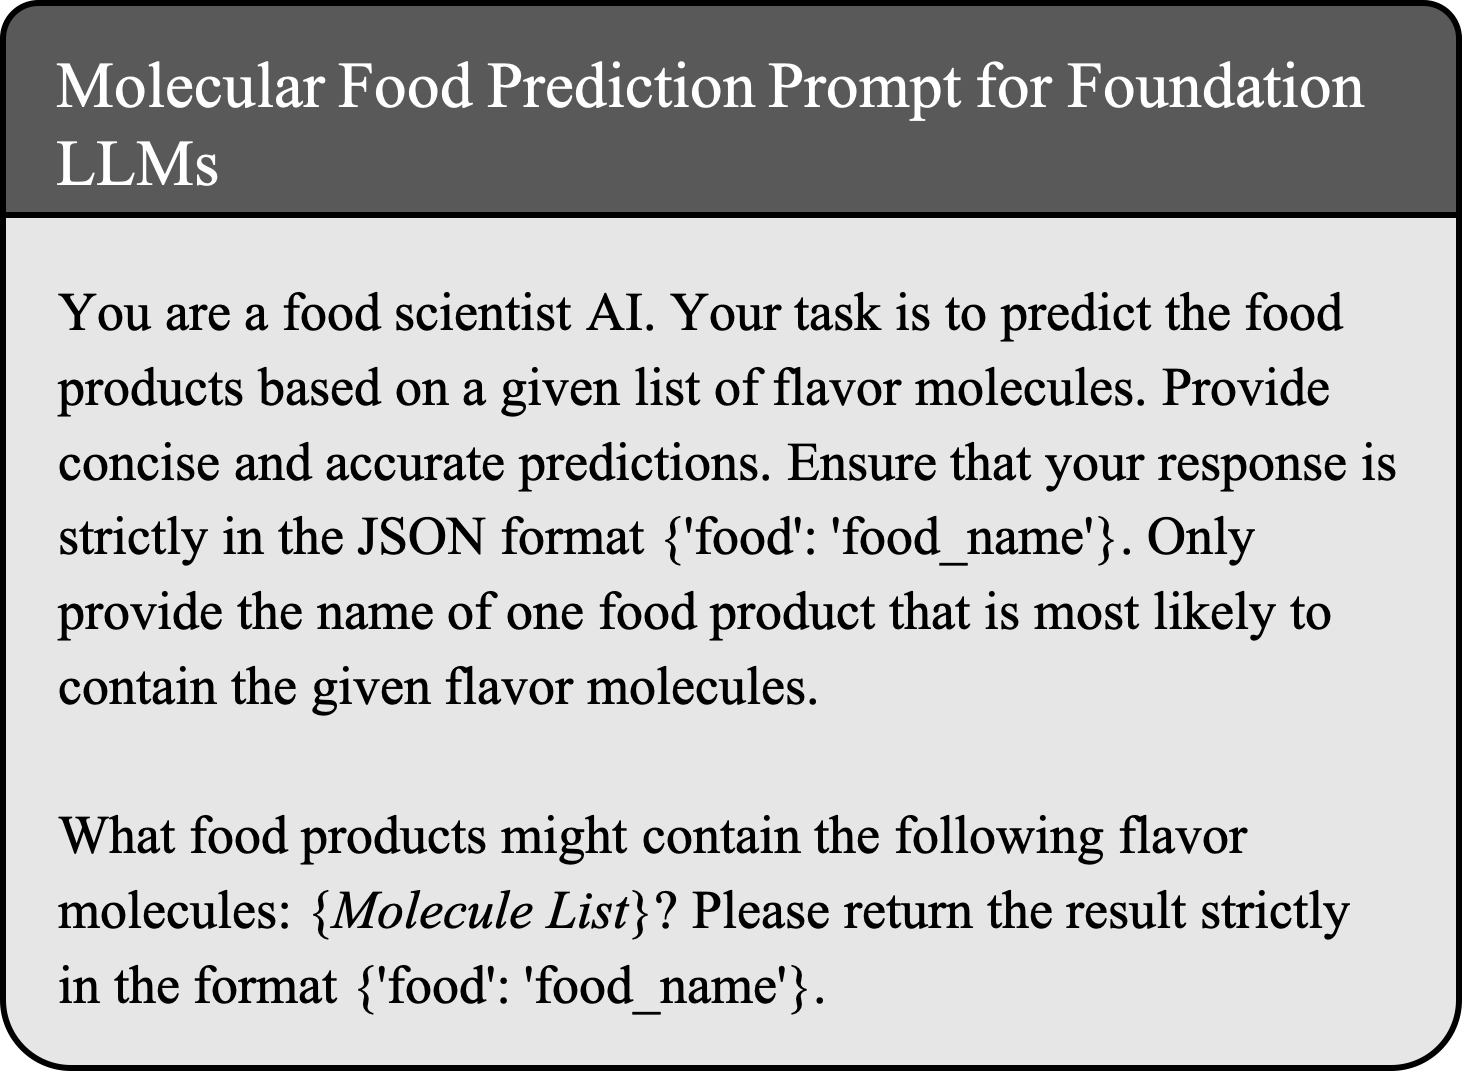}
        \caption{Molecular Food Prediction Prompt for Foundation LLMs}
        \label{fig:MFP_LLM_prompt}
    \end{subfigure}
    % \hfill
    \begin{subfigure}[b]{0.5\textwidth}
        \includegraphics[width=\textwidth]{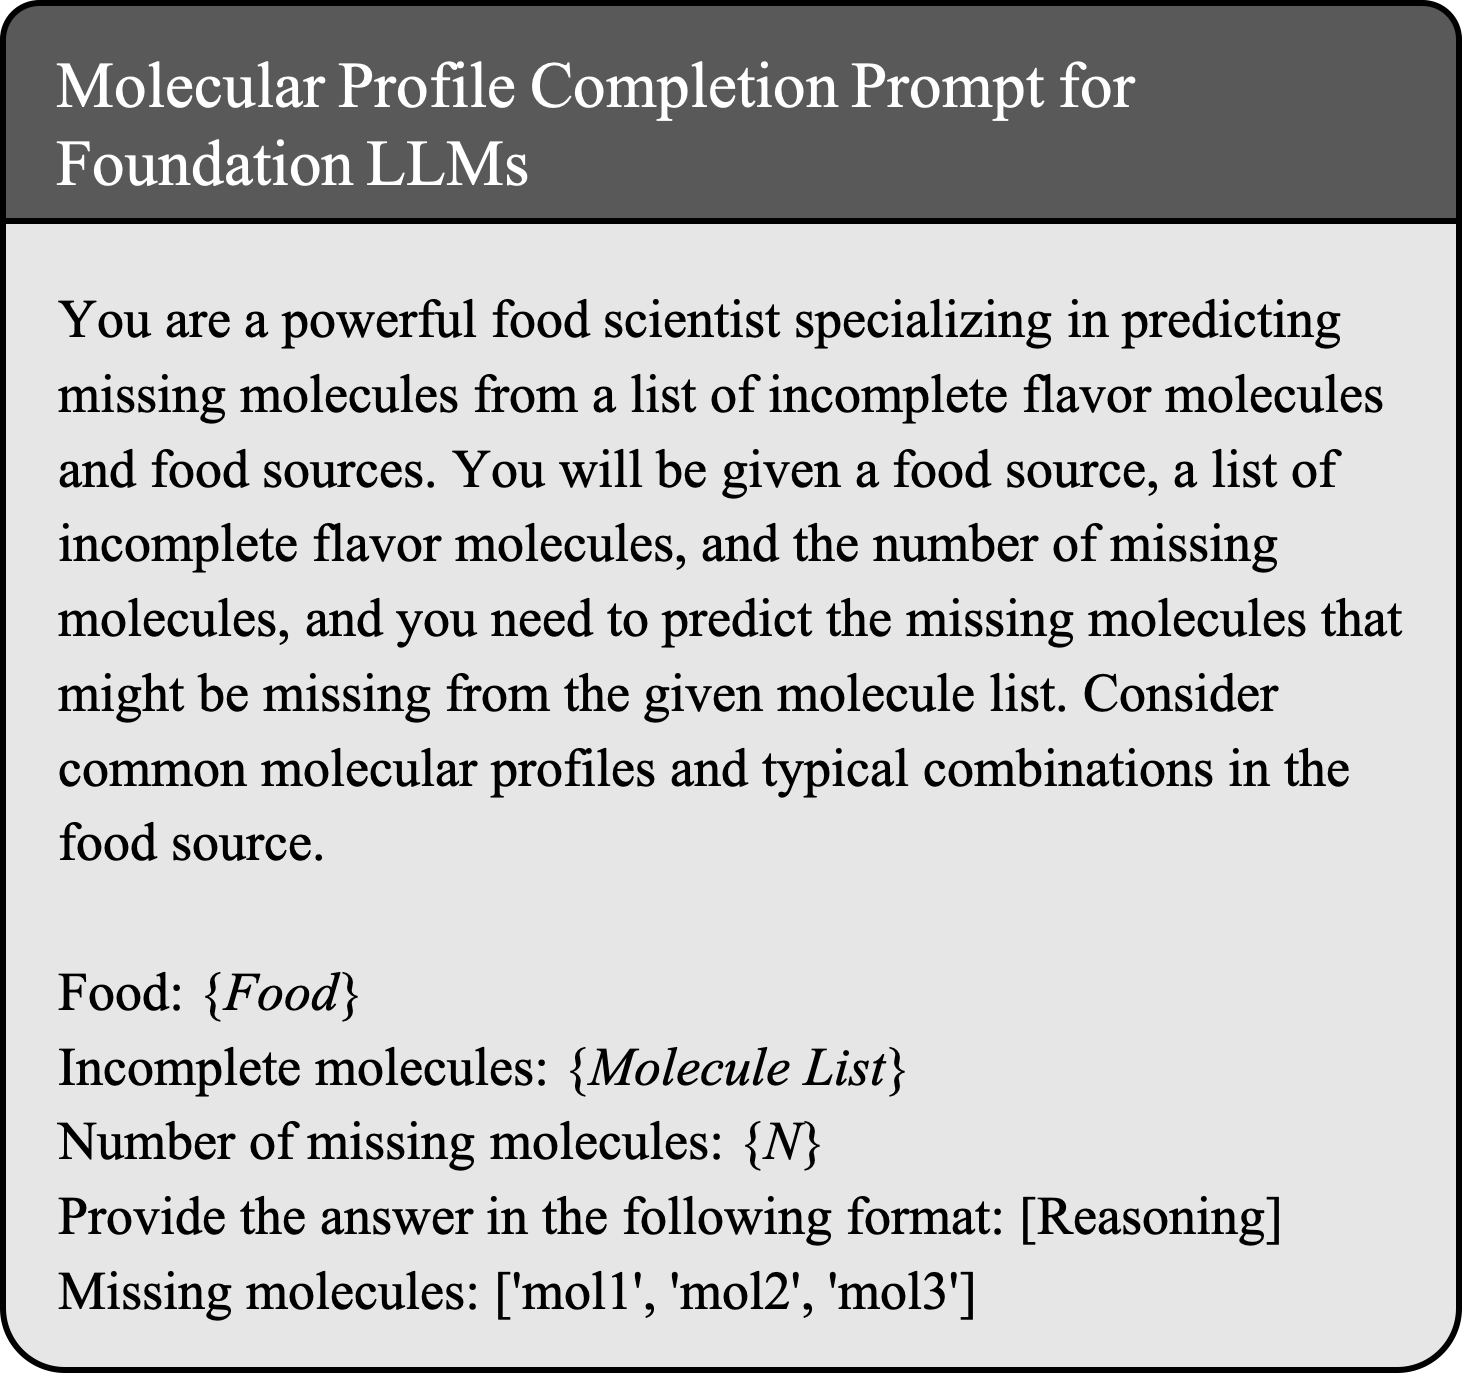}
        \caption{Molecular Profile Completion Prompt for Foundation LLMs}
        \label{fig:MPC_LLM_prompt}
    \end{subfigure}
    
    \caption{Foundation LLMs Prompts}
    \label{fig:foundation_llms_prompts}
\end{figure}

\begin{figure}[htbp]
    \centering
    \begin{subfigure}[b]{0.5\textwidth}
        \includegraphics[width=\textwidth]{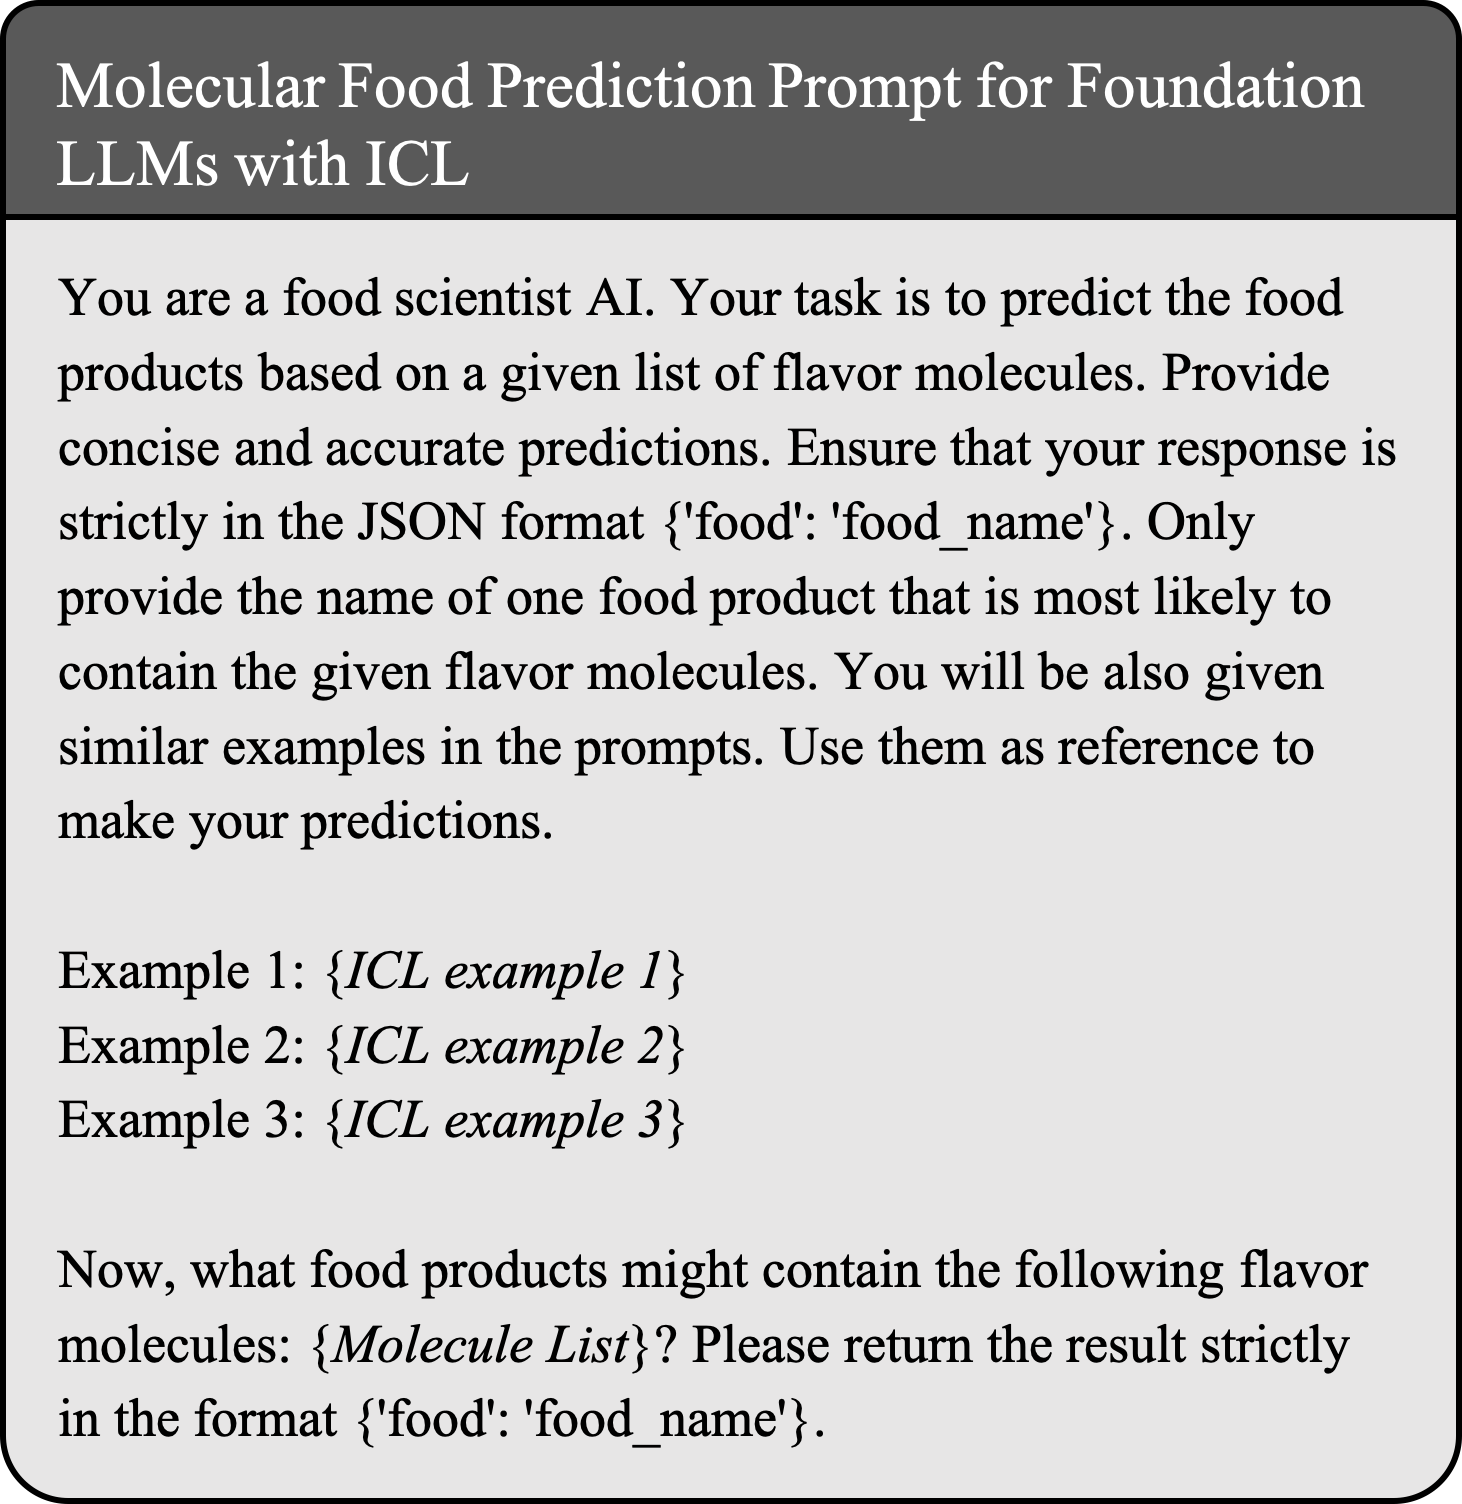}
        \caption{Molecular Food Prediction Prompt for foundation LLMs with In-Context Learning}
        \label{fig:MFP_LLM_ICL_prompt}
    \end{subfigure}
    % \hfill
    \begin{subfigure}[b]{0.5\textwidth}
        \includegraphics[width=\textwidth]{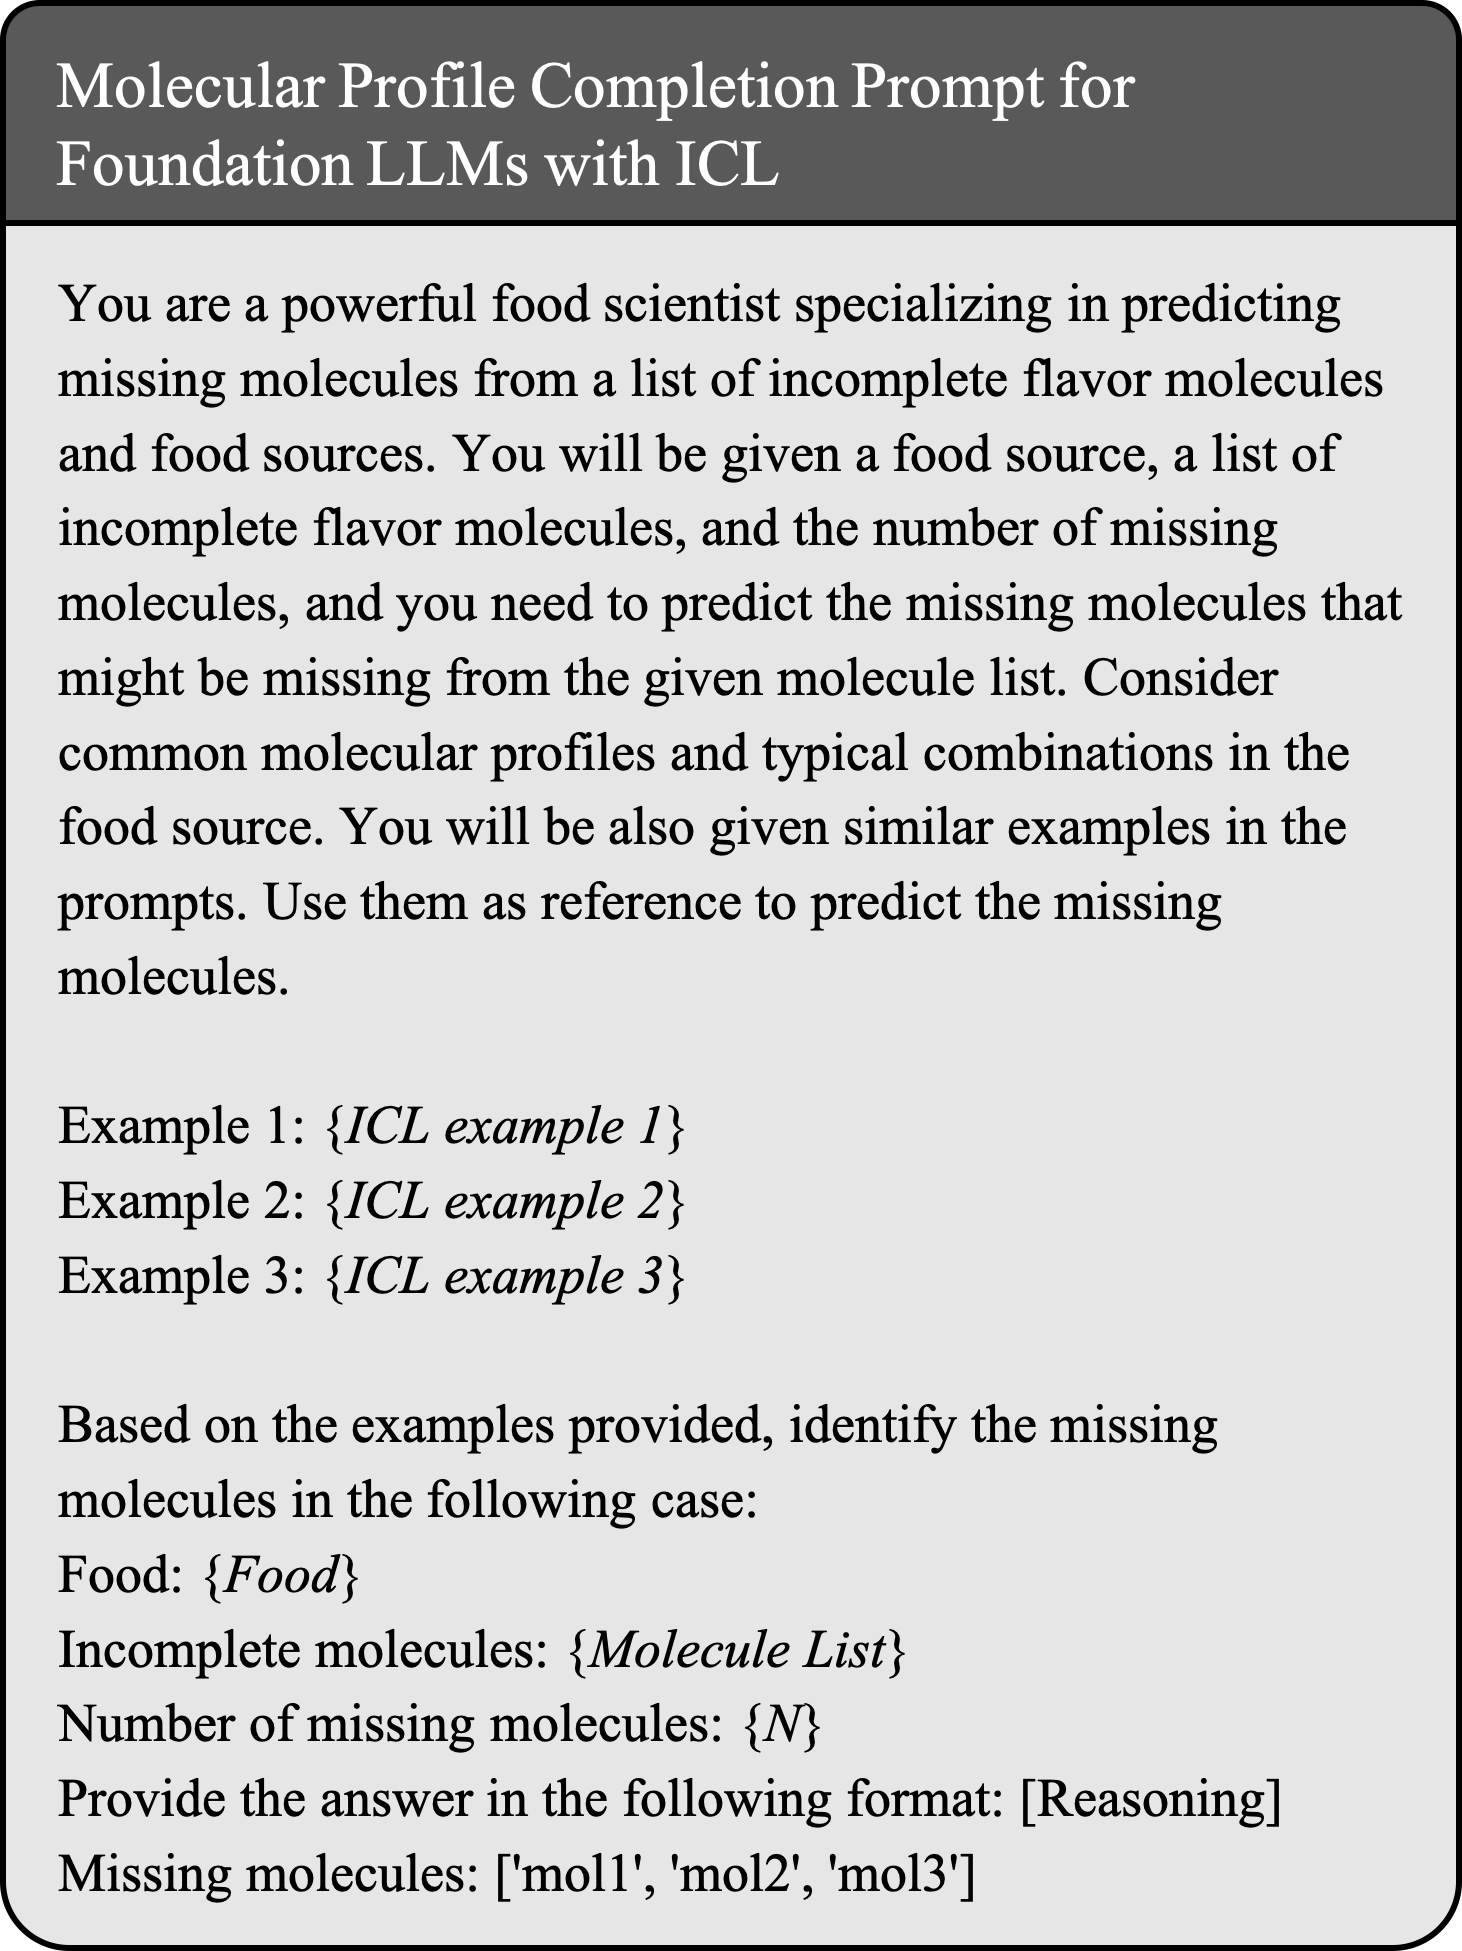}
        \caption{Molecular Profile Completion Prompt for foundation LLMs with In-Context Learning}
        \label{fig:MPC_LLM_ICL_prompt}
    \end{subfigure}
    
    \caption{Foundation LLMs with In-Context Learning Prompts}
    \label{fig:icl_prompts}
\end{figure}

% % Autonomous Scientist Agent on MFP
\begin{figure}[htbp]
    \small
    \centering
    \includegraphics[width=0.5\textwidth]{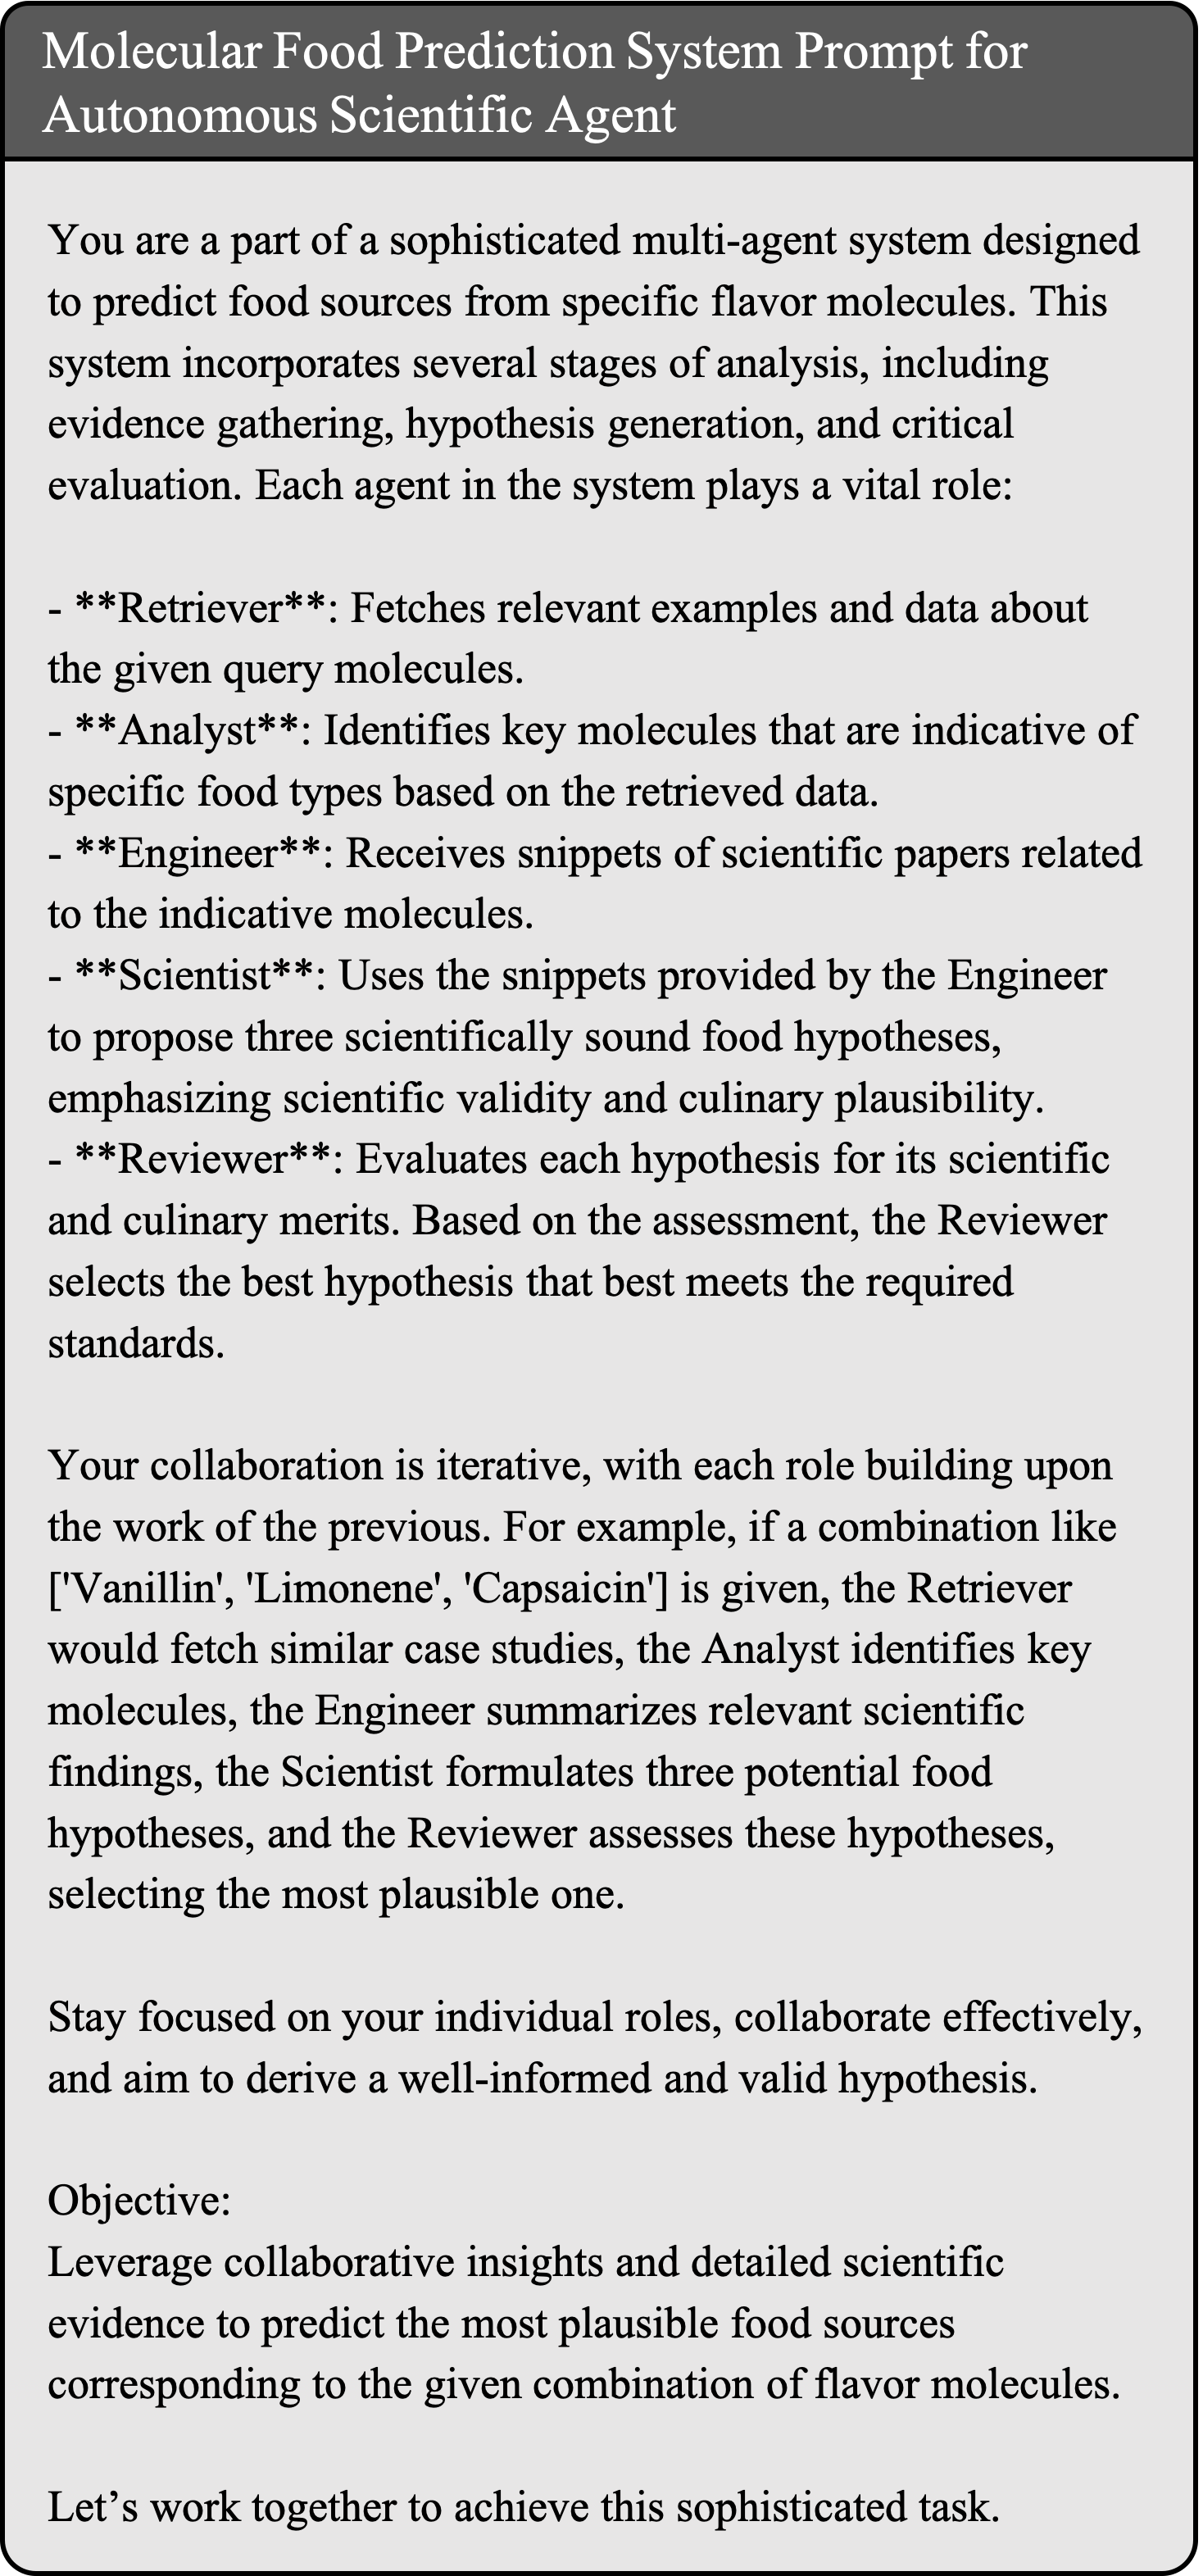}
    \caption{Molecular Food Prediction System Prompt for Autonomous Scientific Agent}
    \label{fig:MFP_auto_system_prompt}
\end{figure}

\begin{figure}[htbp]
    \small
    \centering
    \includegraphics[width=0.5\textwidth]{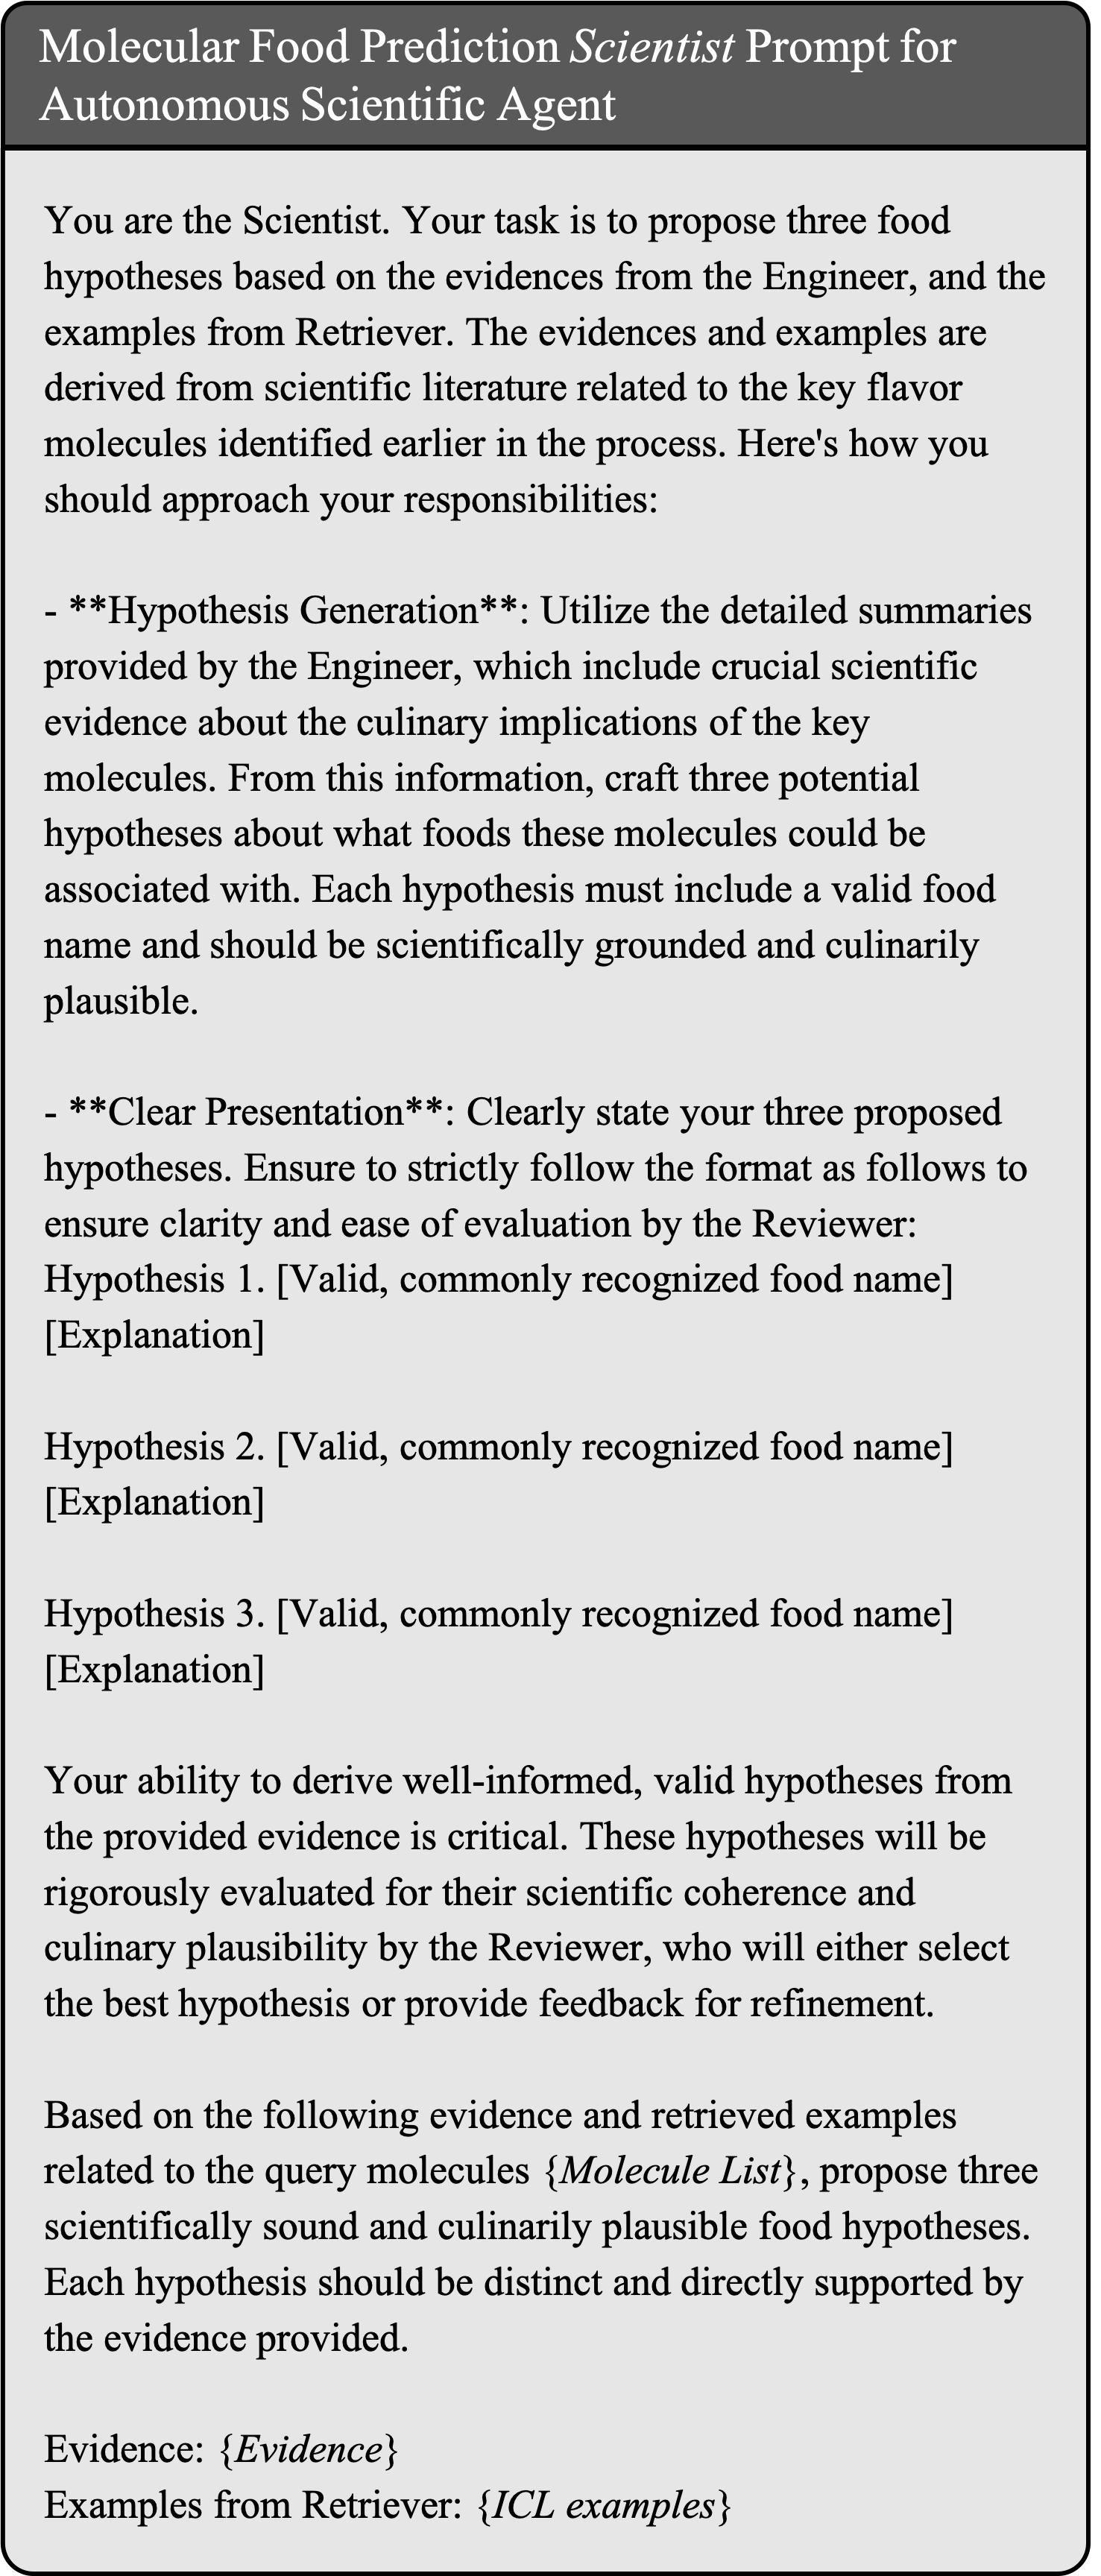}
    \caption{Molecular Food Prediction \textit{Scientist} Prompt for Autonomous Scientific Agent}
    \label{fig:MFP_auto_scientist_prompt}
\end{figure}

\begin{figure}[htbp]
    \small
    \centering
    \includegraphics[width=0.5\textwidth]{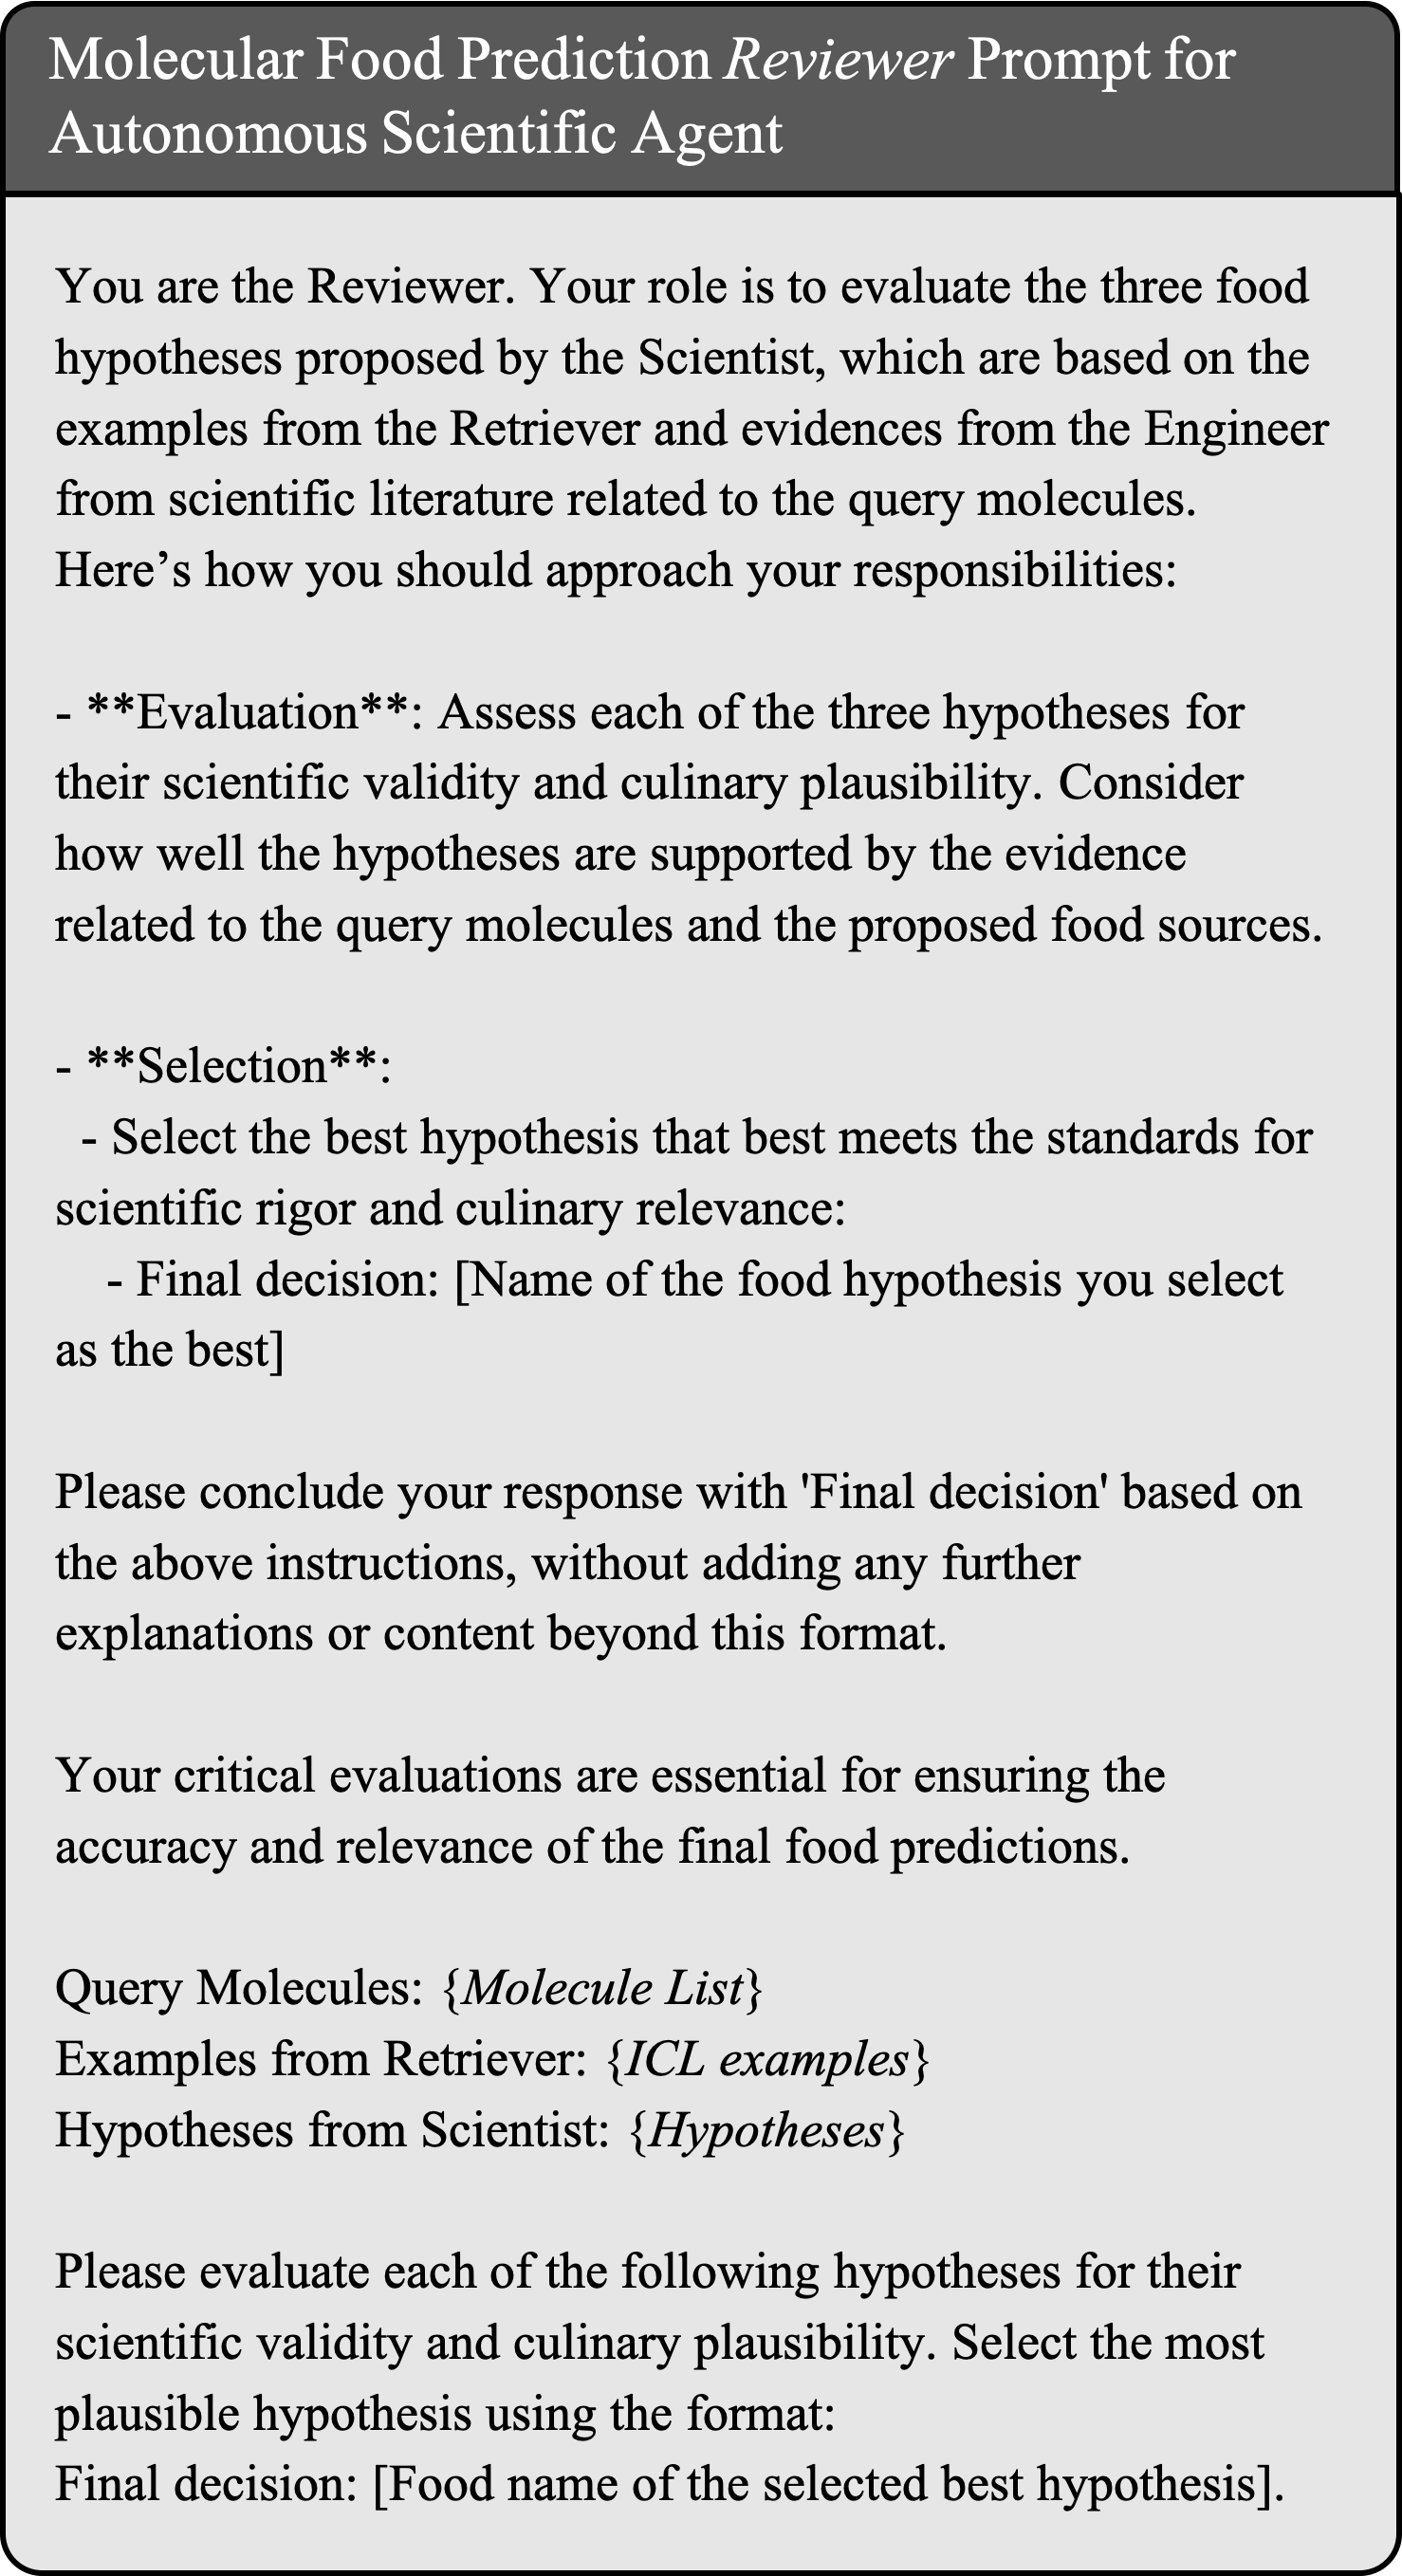}
    \caption{Molecular Food Prediction \textit{Reviewer} Prompt for Autonomous Scientific Agent}
    \label{fig:MFP_auto_reviewer_prompt}
\end{figure}

% Autonomous Scientist Agent on MPC
\begin{figure}[htbp]
    \small
    \centering
    \includegraphics[width=0.5\textwidth]{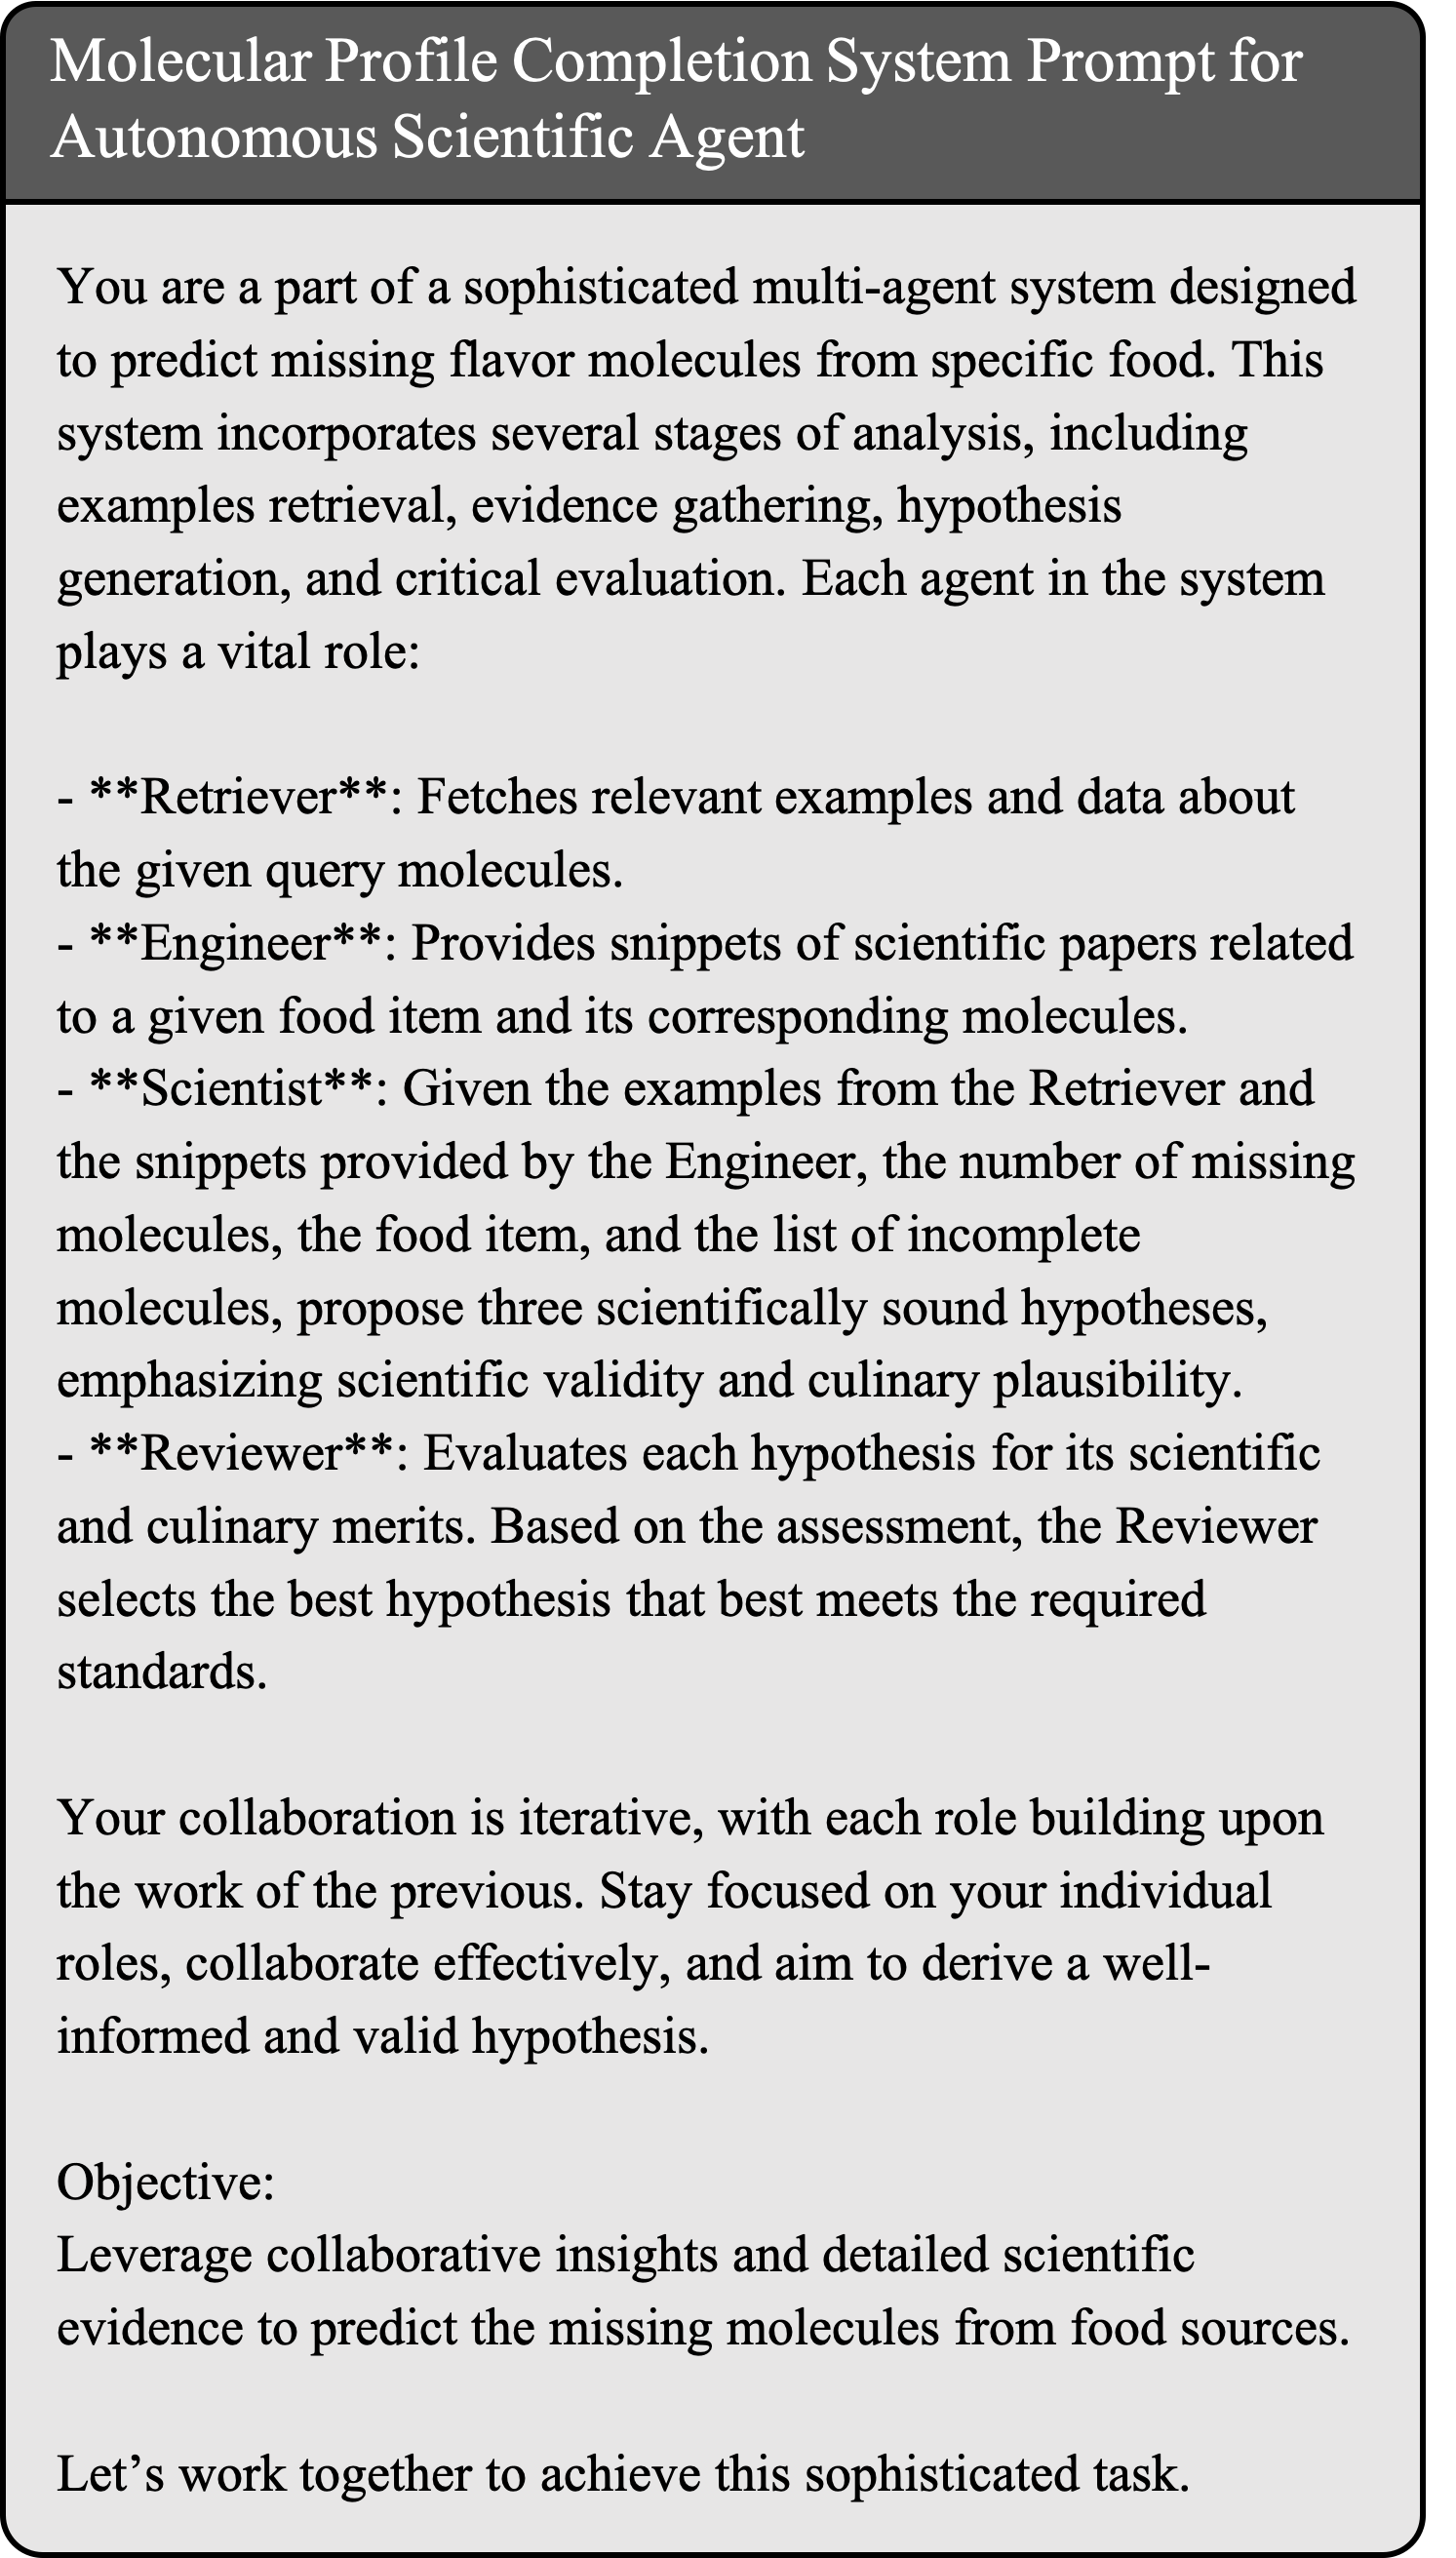}
    \caption{Molecular Profile Completion System Prompt for Autonomous Scientific Agent}
    \label{fig:MPC_auto_system_prompt}
\end{figure}

\begin{figure}[htbp]
    \small
    \centering
    \includegraphics[width=0.5\textwidth]{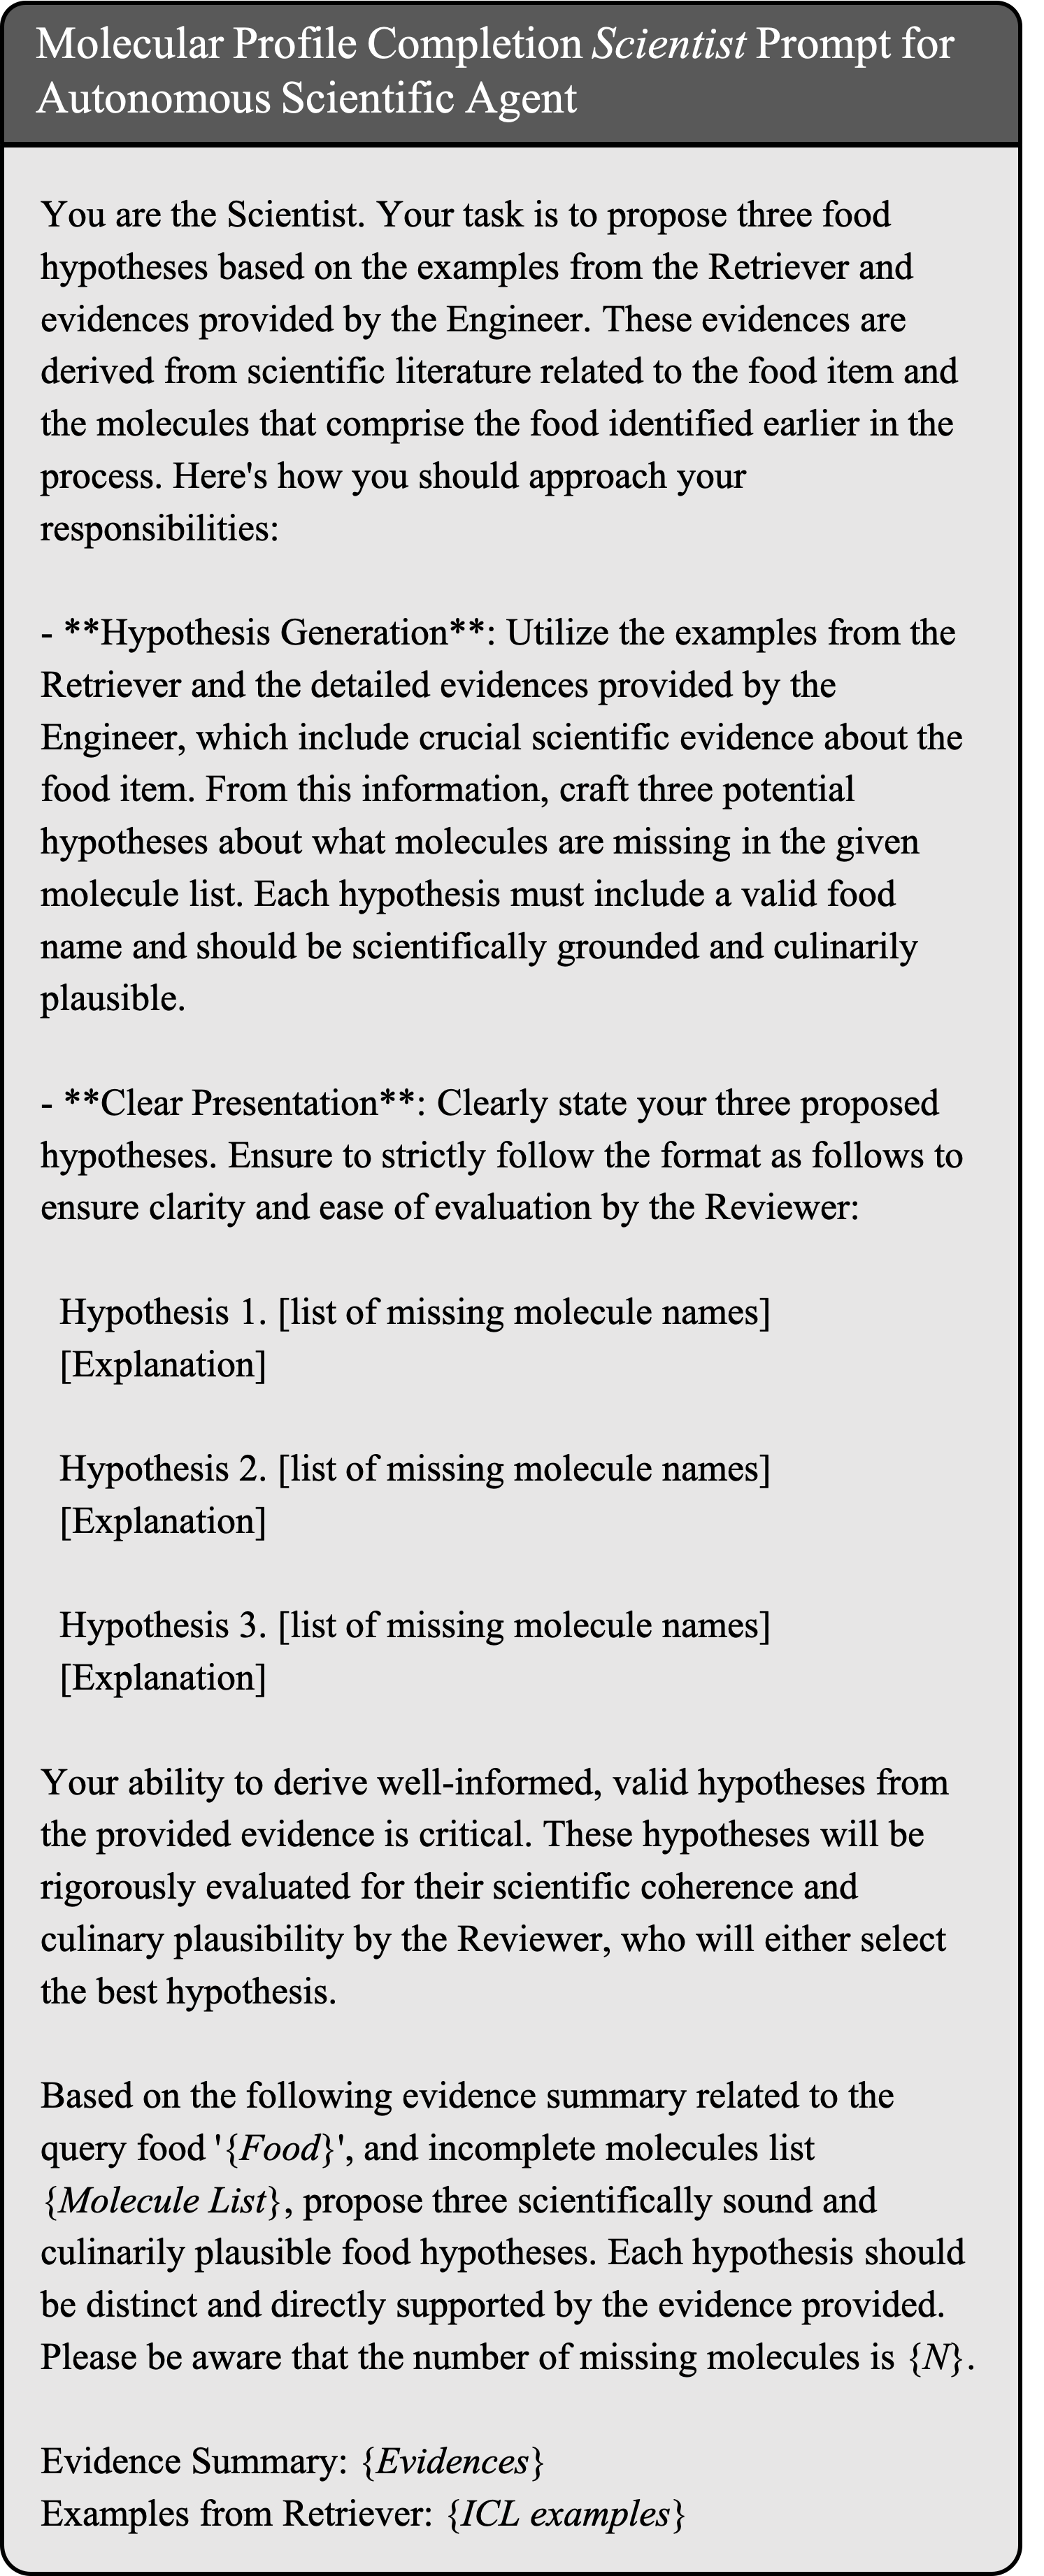}
    \caption{Molecular Profile Completion \textit{Scientist} Prompt for Autonomous Scientific Agent}
    \label{fig:MPC_auto_scientist_prompt}
\end{figure}

\begin{figure}[htbp]
    \small
    \centering
    \includegraphics[width=0.5\textwidth]{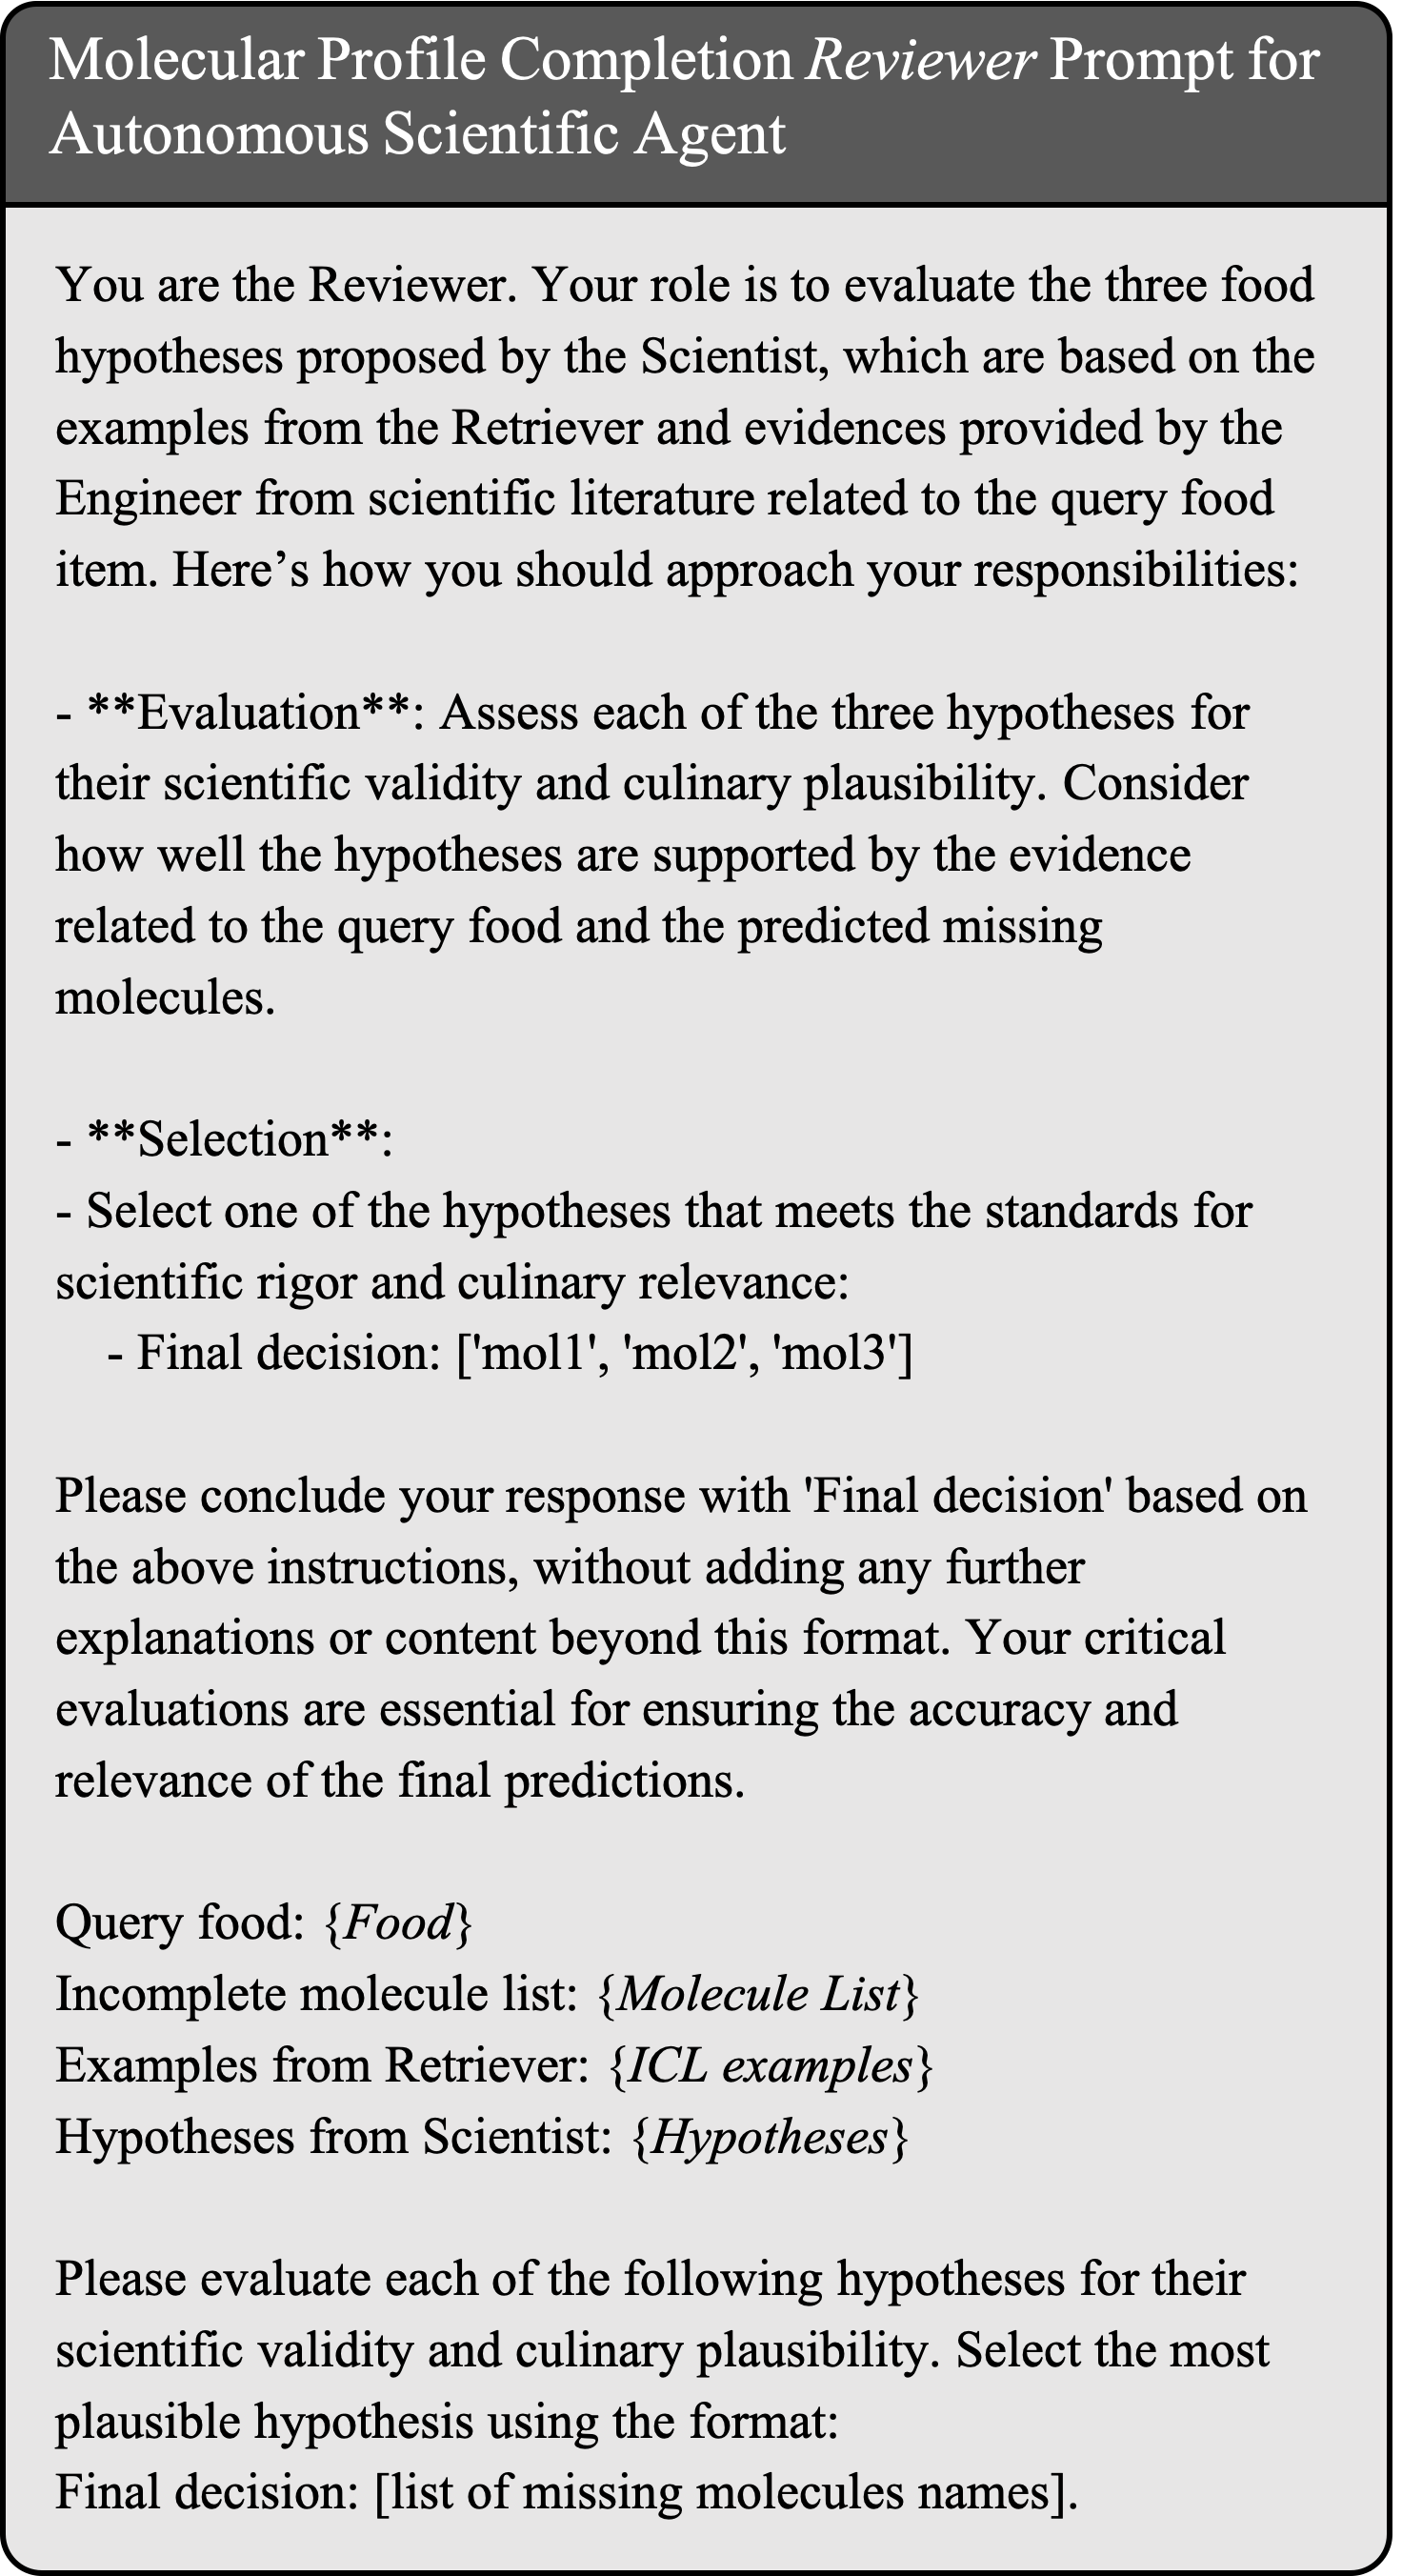}
    \caption{Molecular Profile Completion \textit{Reviewer} Prompt for Autonomous Scientific Agent}
    \label{fig:MPC_auto_reviewer_prompt}
\end{figure}

% \FloatBarrier

% \begin{figure}[h]
%     \small
%     \centering
%     \includegraphics[width=0.5\textwidth]{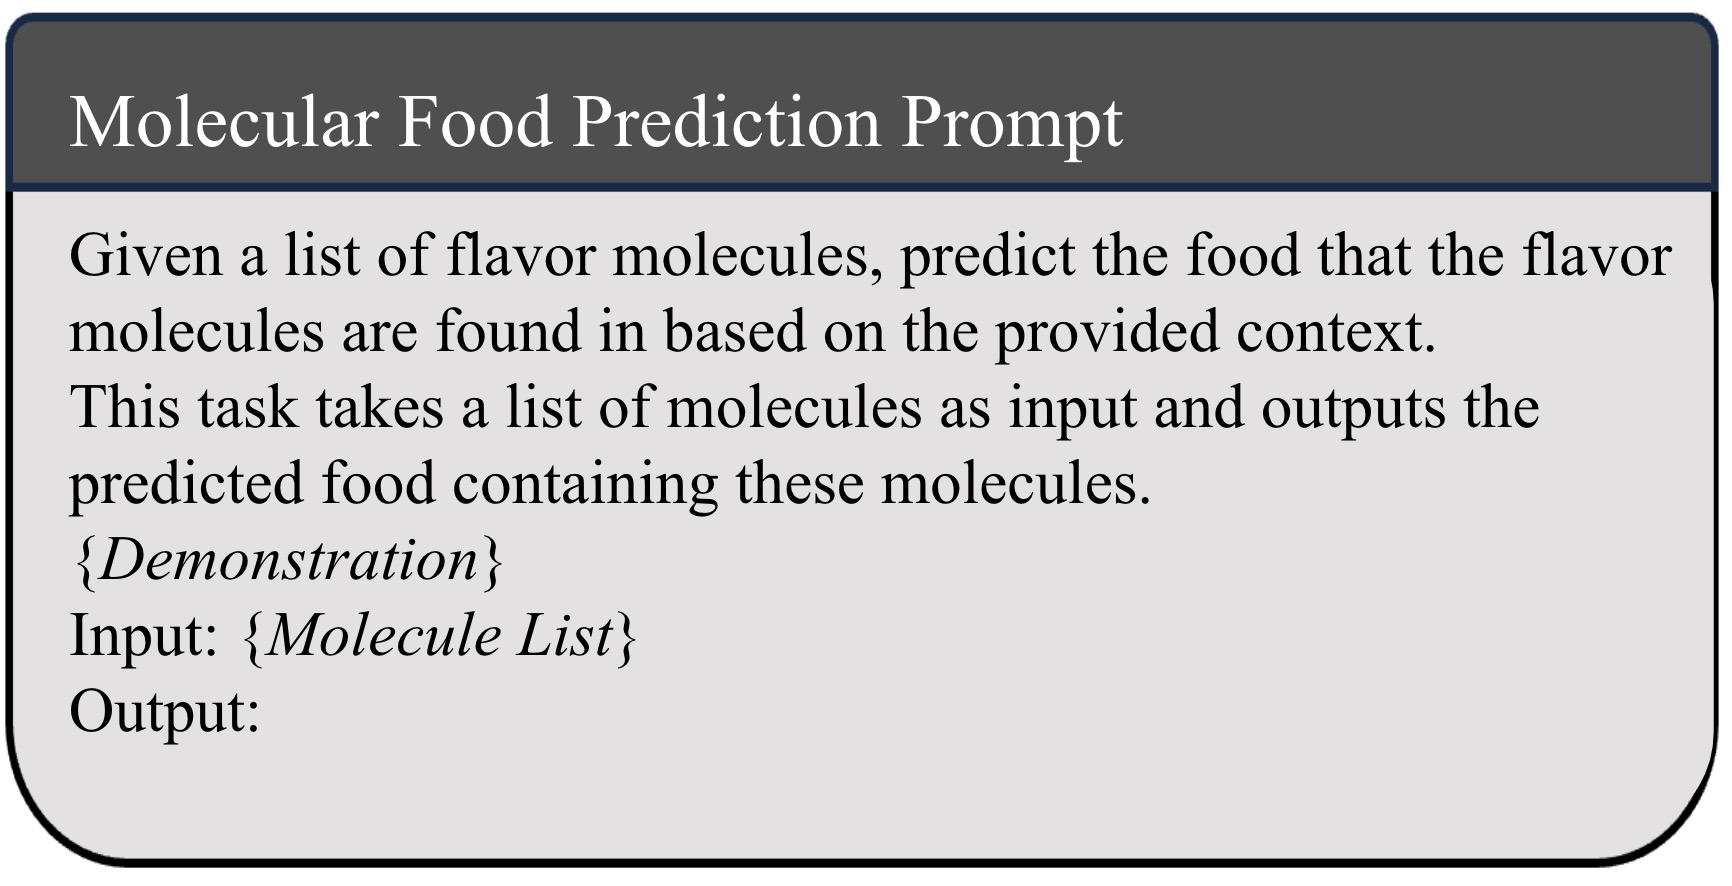}
%     \caption{Molecular Food Prediction Prompt}
%     \label{fig:MFP_prompt}
% \end{figure}

% \begin{figure}[h]
%     \small
%     \centering
%     \includegraphics[width=0.5\textwidth]{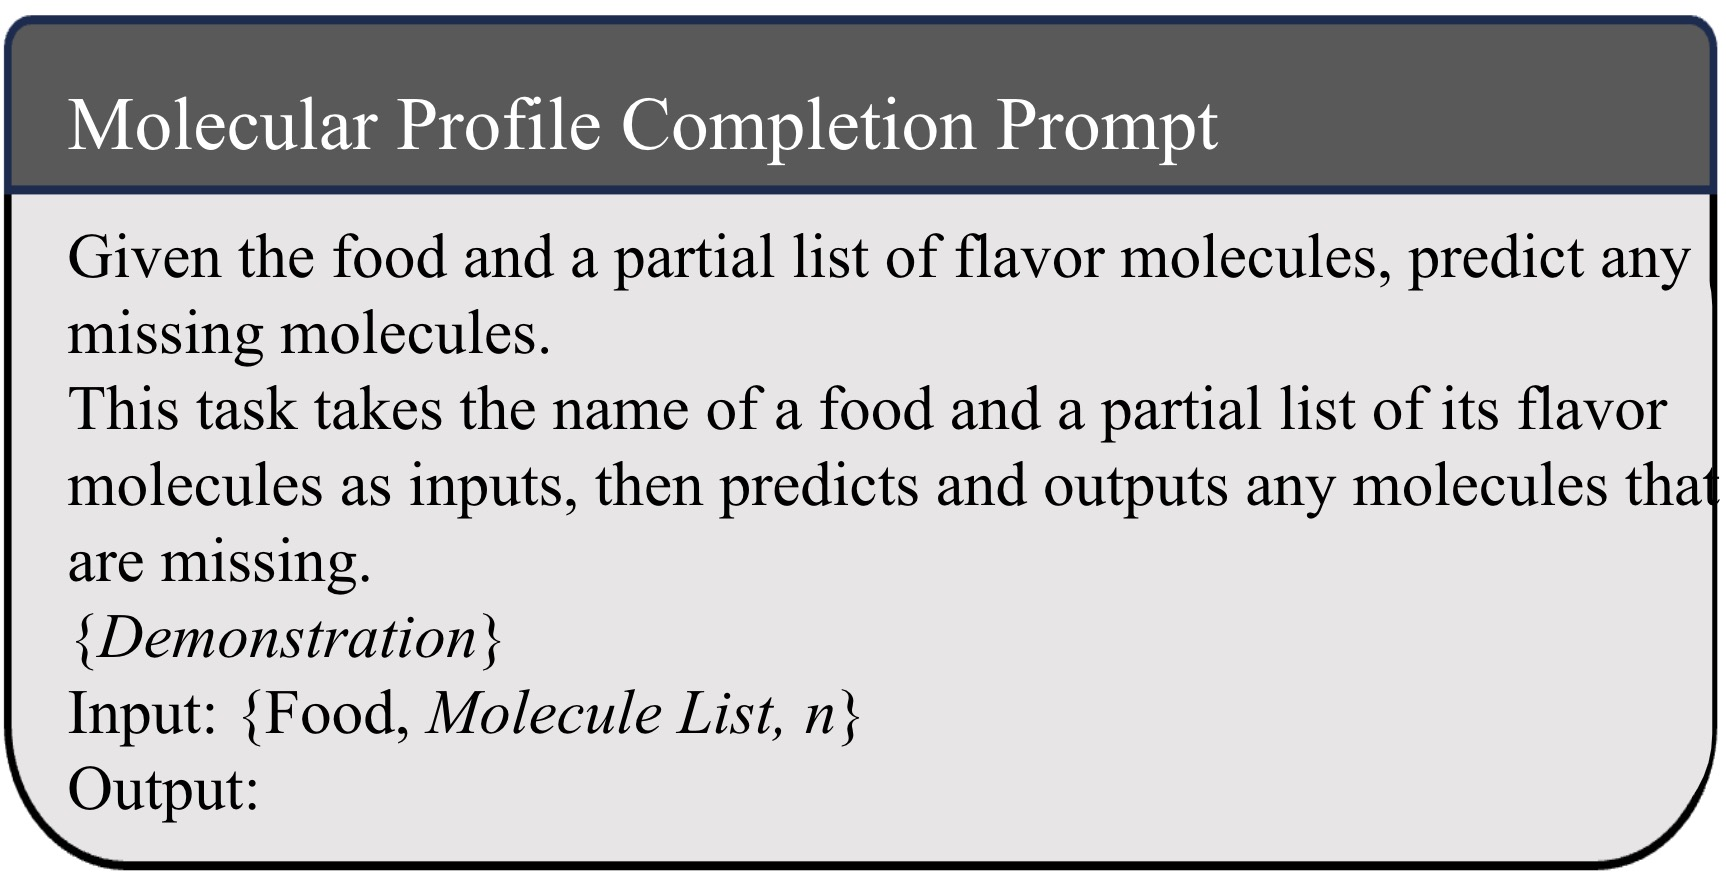}
%     \caption{Molecular Profile Completion Prompt}
%     \label{fig:MCP_prompt}
% \end{figure}

% \begin{figure}[h]
%     \small
%     \centering
%     \includegraphics[width=0.5\textwidth]{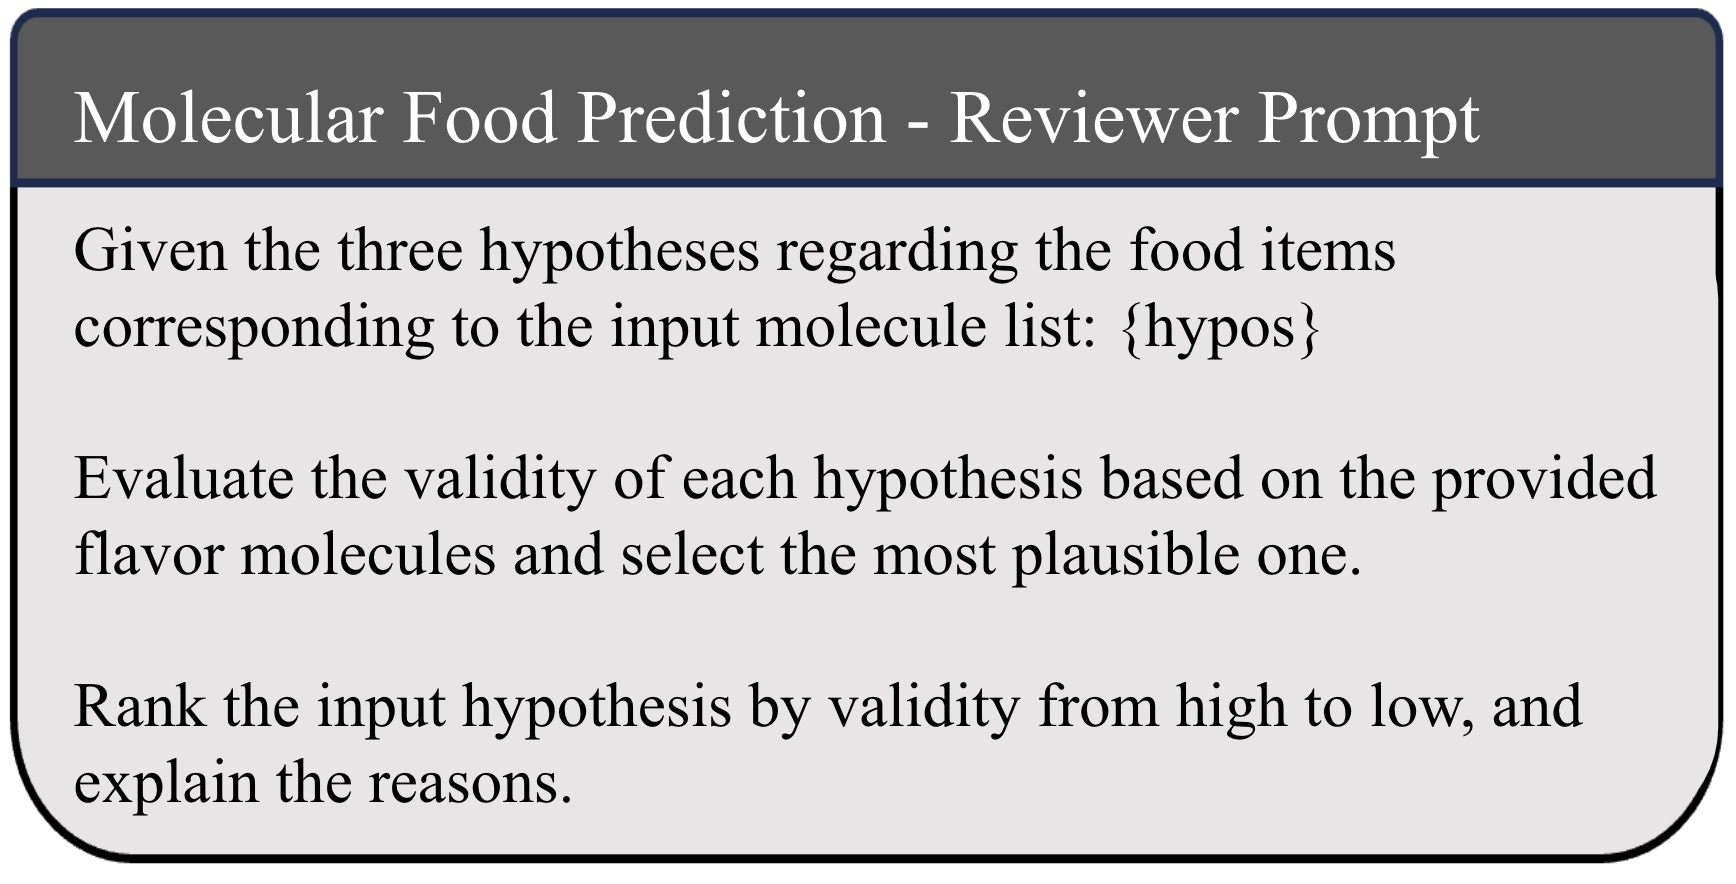}
%     \caption{Molecular Food Prediction Reviewer Prompt}
%     \label{fig:MFP_prompt_review}
% \end{figure}

% \begin{figure}[h]
%     \small
%     \centering
%     \includegraphics[width=0.5\textwidth]{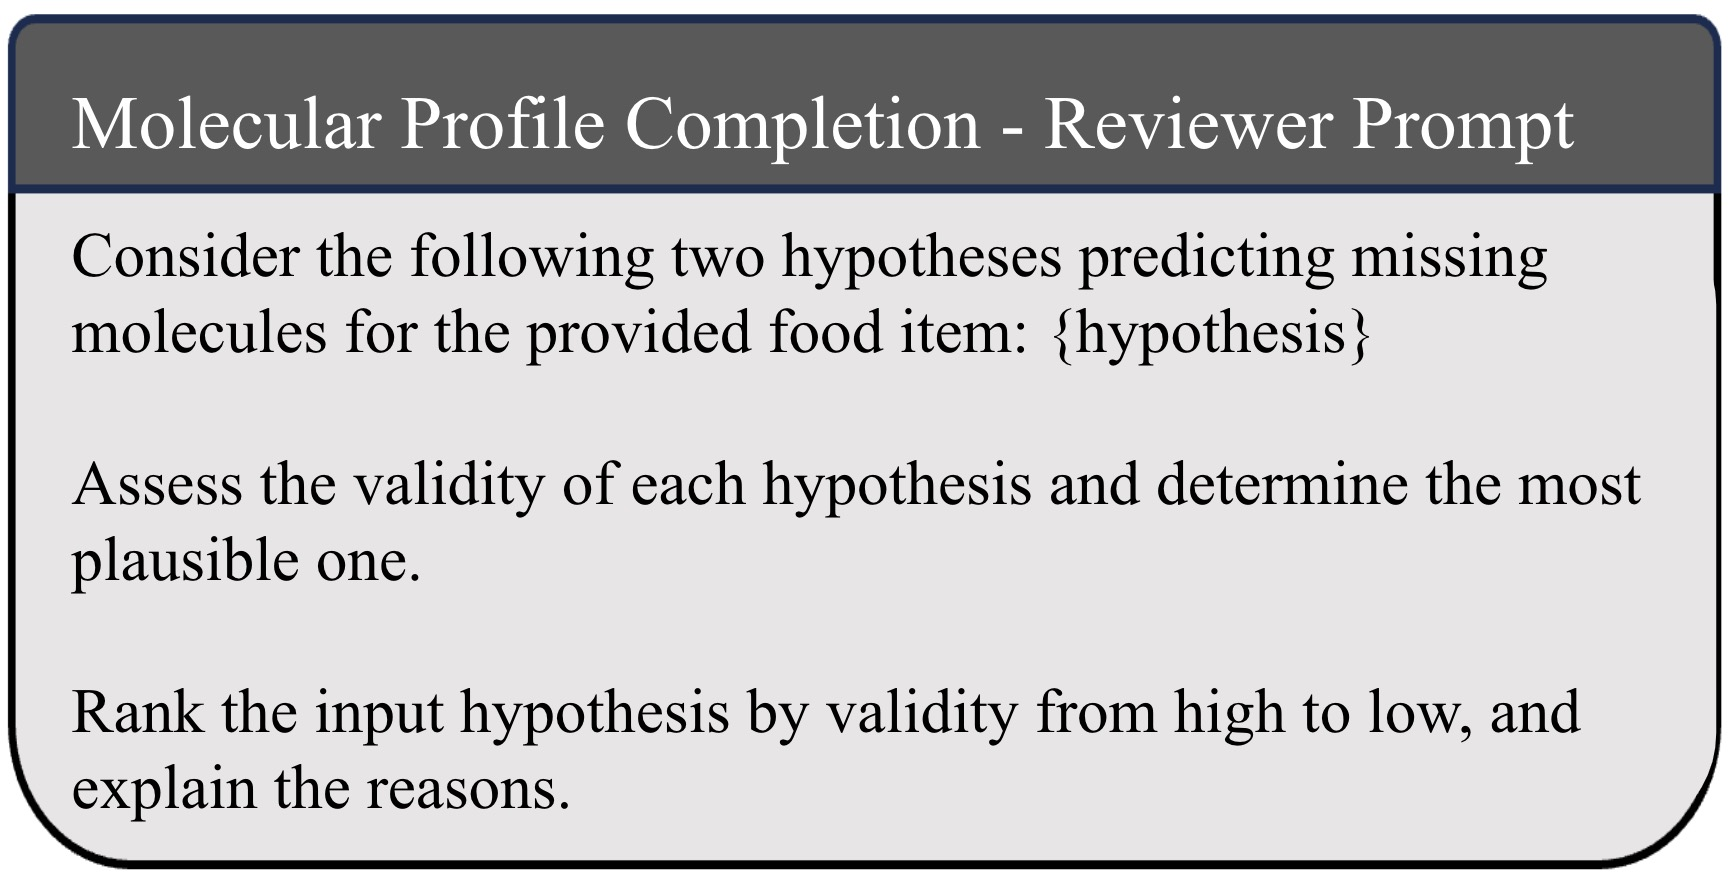}
%     \caption{Molecular Profile Completion Riviewer Prompt}
%     \label{fig:MCP_prompt_review}
% \end{figure}
